# Supplementary material for: Distributed Weighted Parameter Averaging for SVM Training on Big Data
Source: arXiv:1509.09030 source file (2015-09-30)
Supplement: Supplementary file 1 [file appendix1.tex]

\section*{Appendix A}
\textbf{Convergence of primal residuals}\\
  \begin{figure}[!ht] 
   \captionsetup[subfigure]{labelformat=empty}
  \begin{center}
   \subfloat[]{%[50 partitions]{%[10 partitions]
   \includegraphics[width=0.34\linewidth]{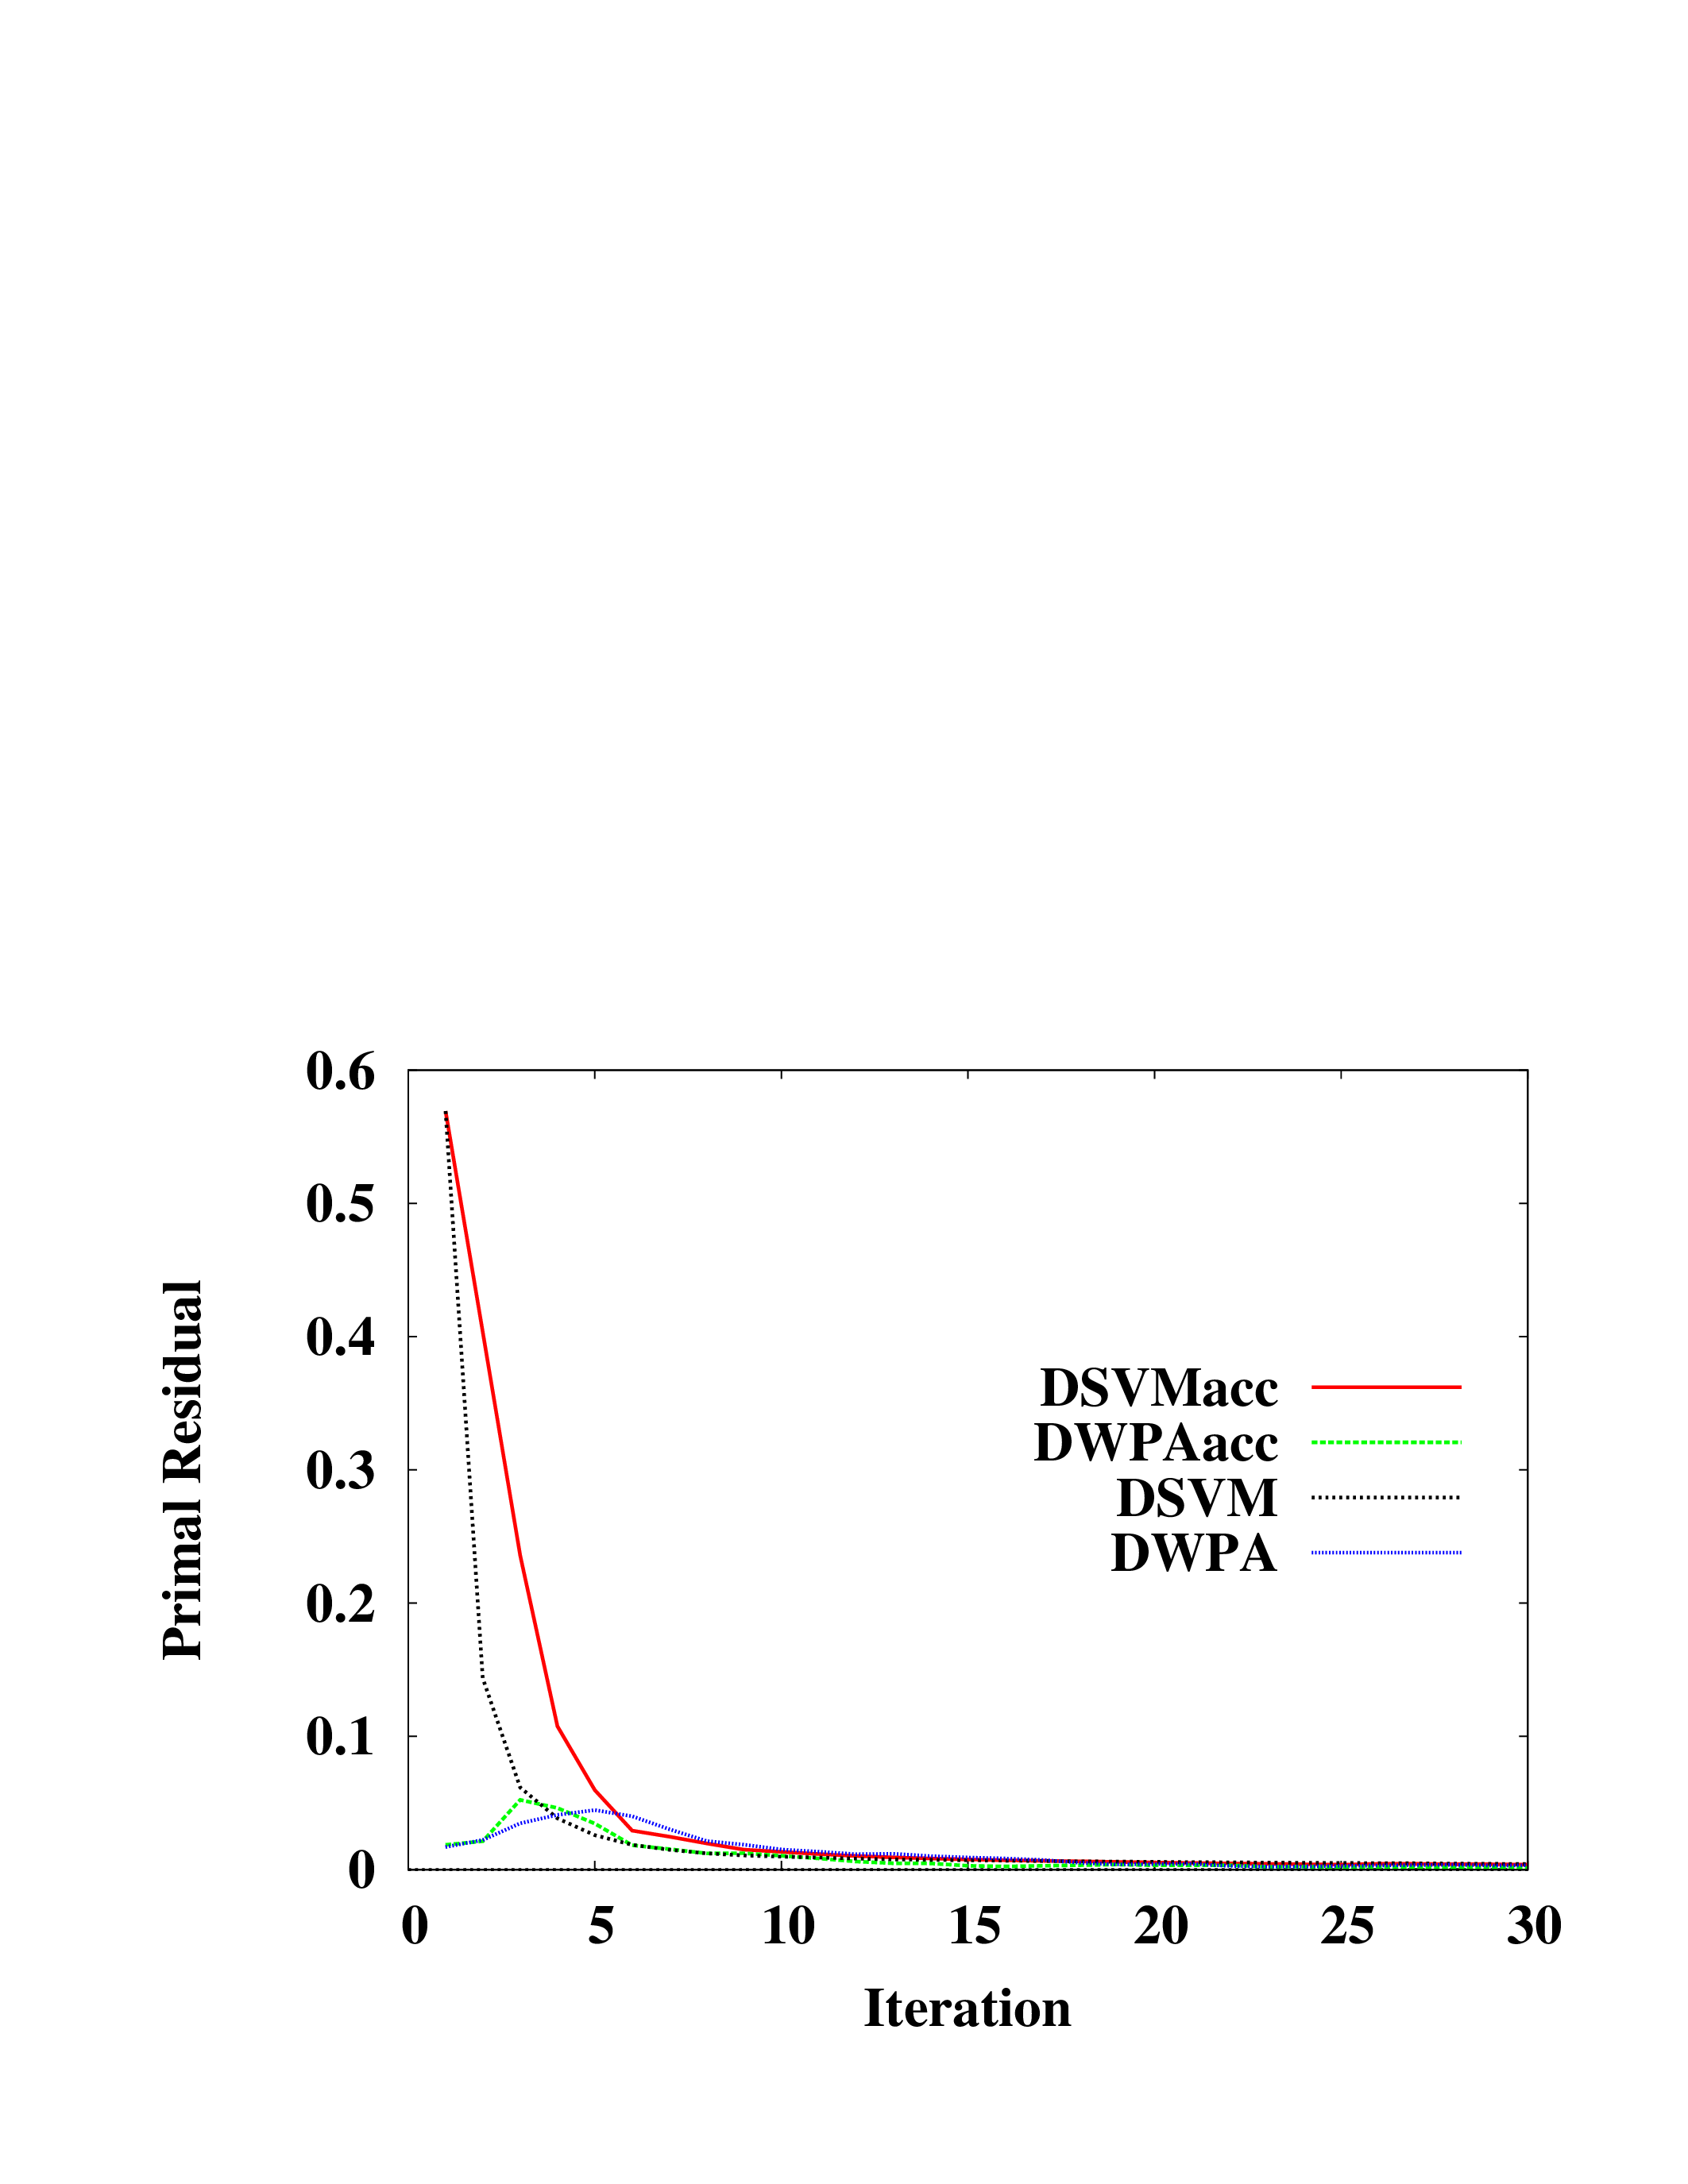}
    }
   \hspace{-.45cm}
    \subfloat[]{%[100 partitions]{%[10 partitions]
   \includegraphics[width=0.34\linewidth]{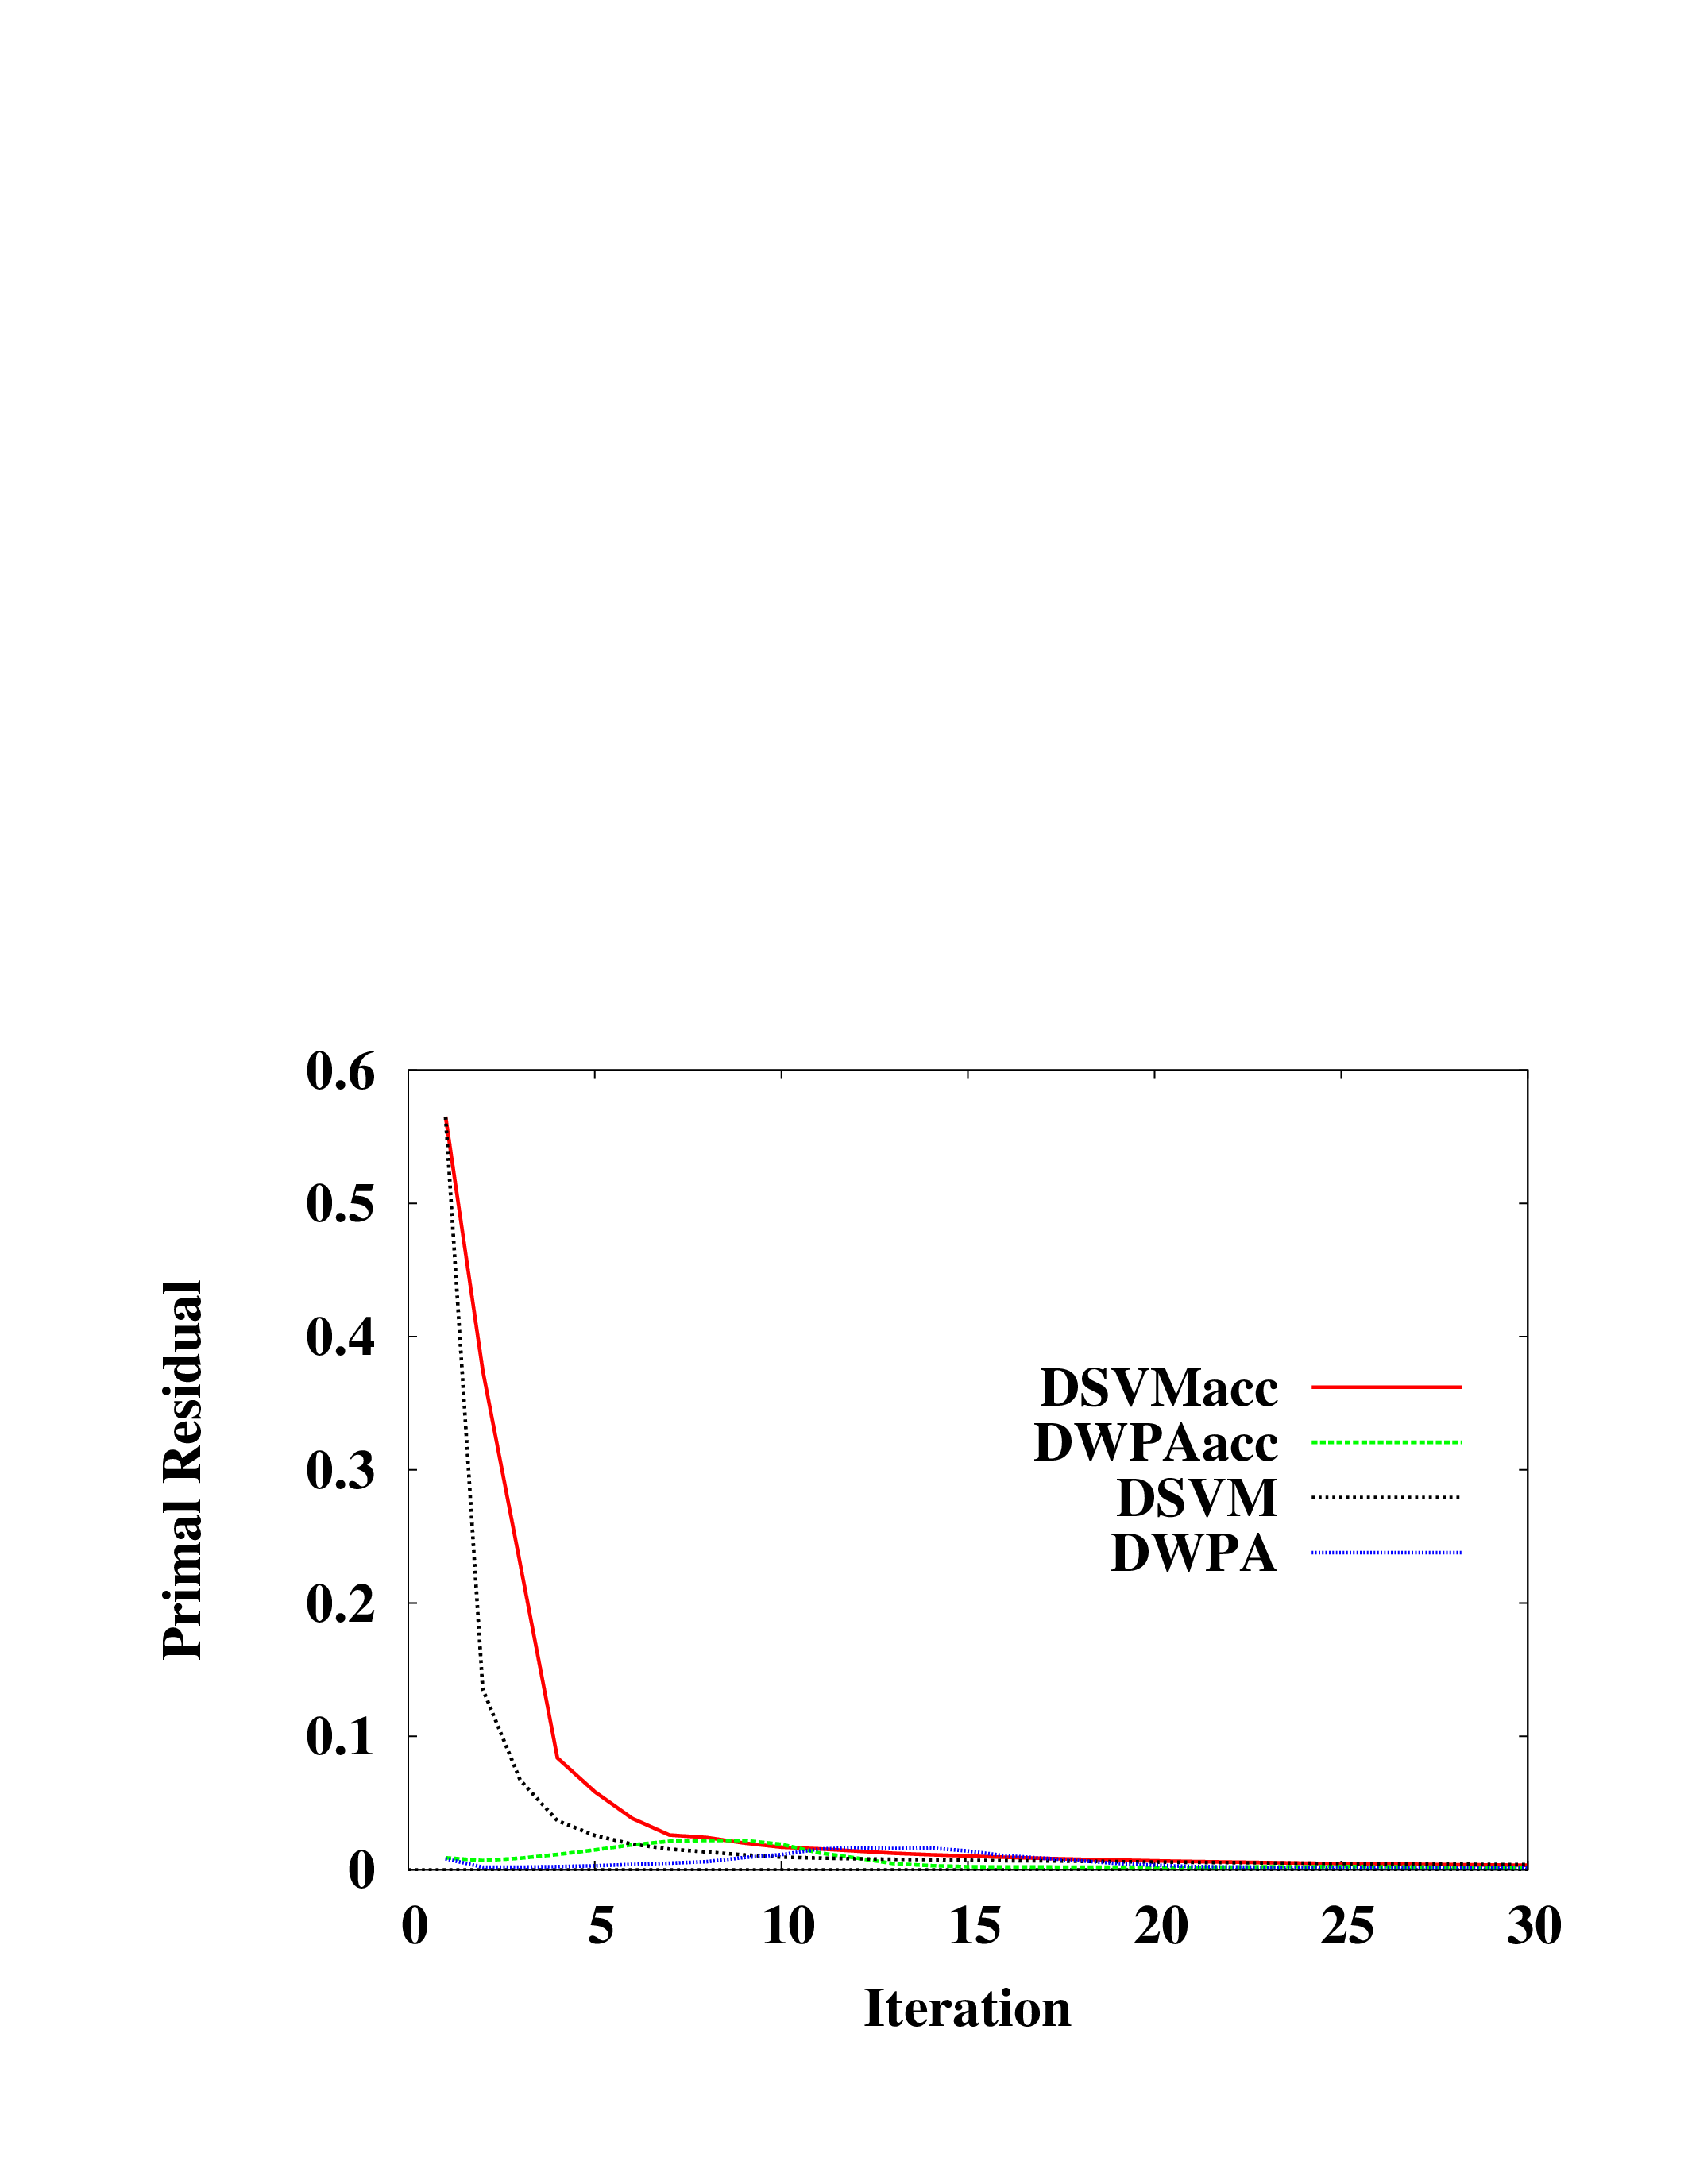}
    }
 %   \vspace{-1.6cm}
   \hspace{-.45cm}
    \subfloat[]{%[200 partitions]{%[10 partitions]
   \includegraphics[width=0.34\linewidth]{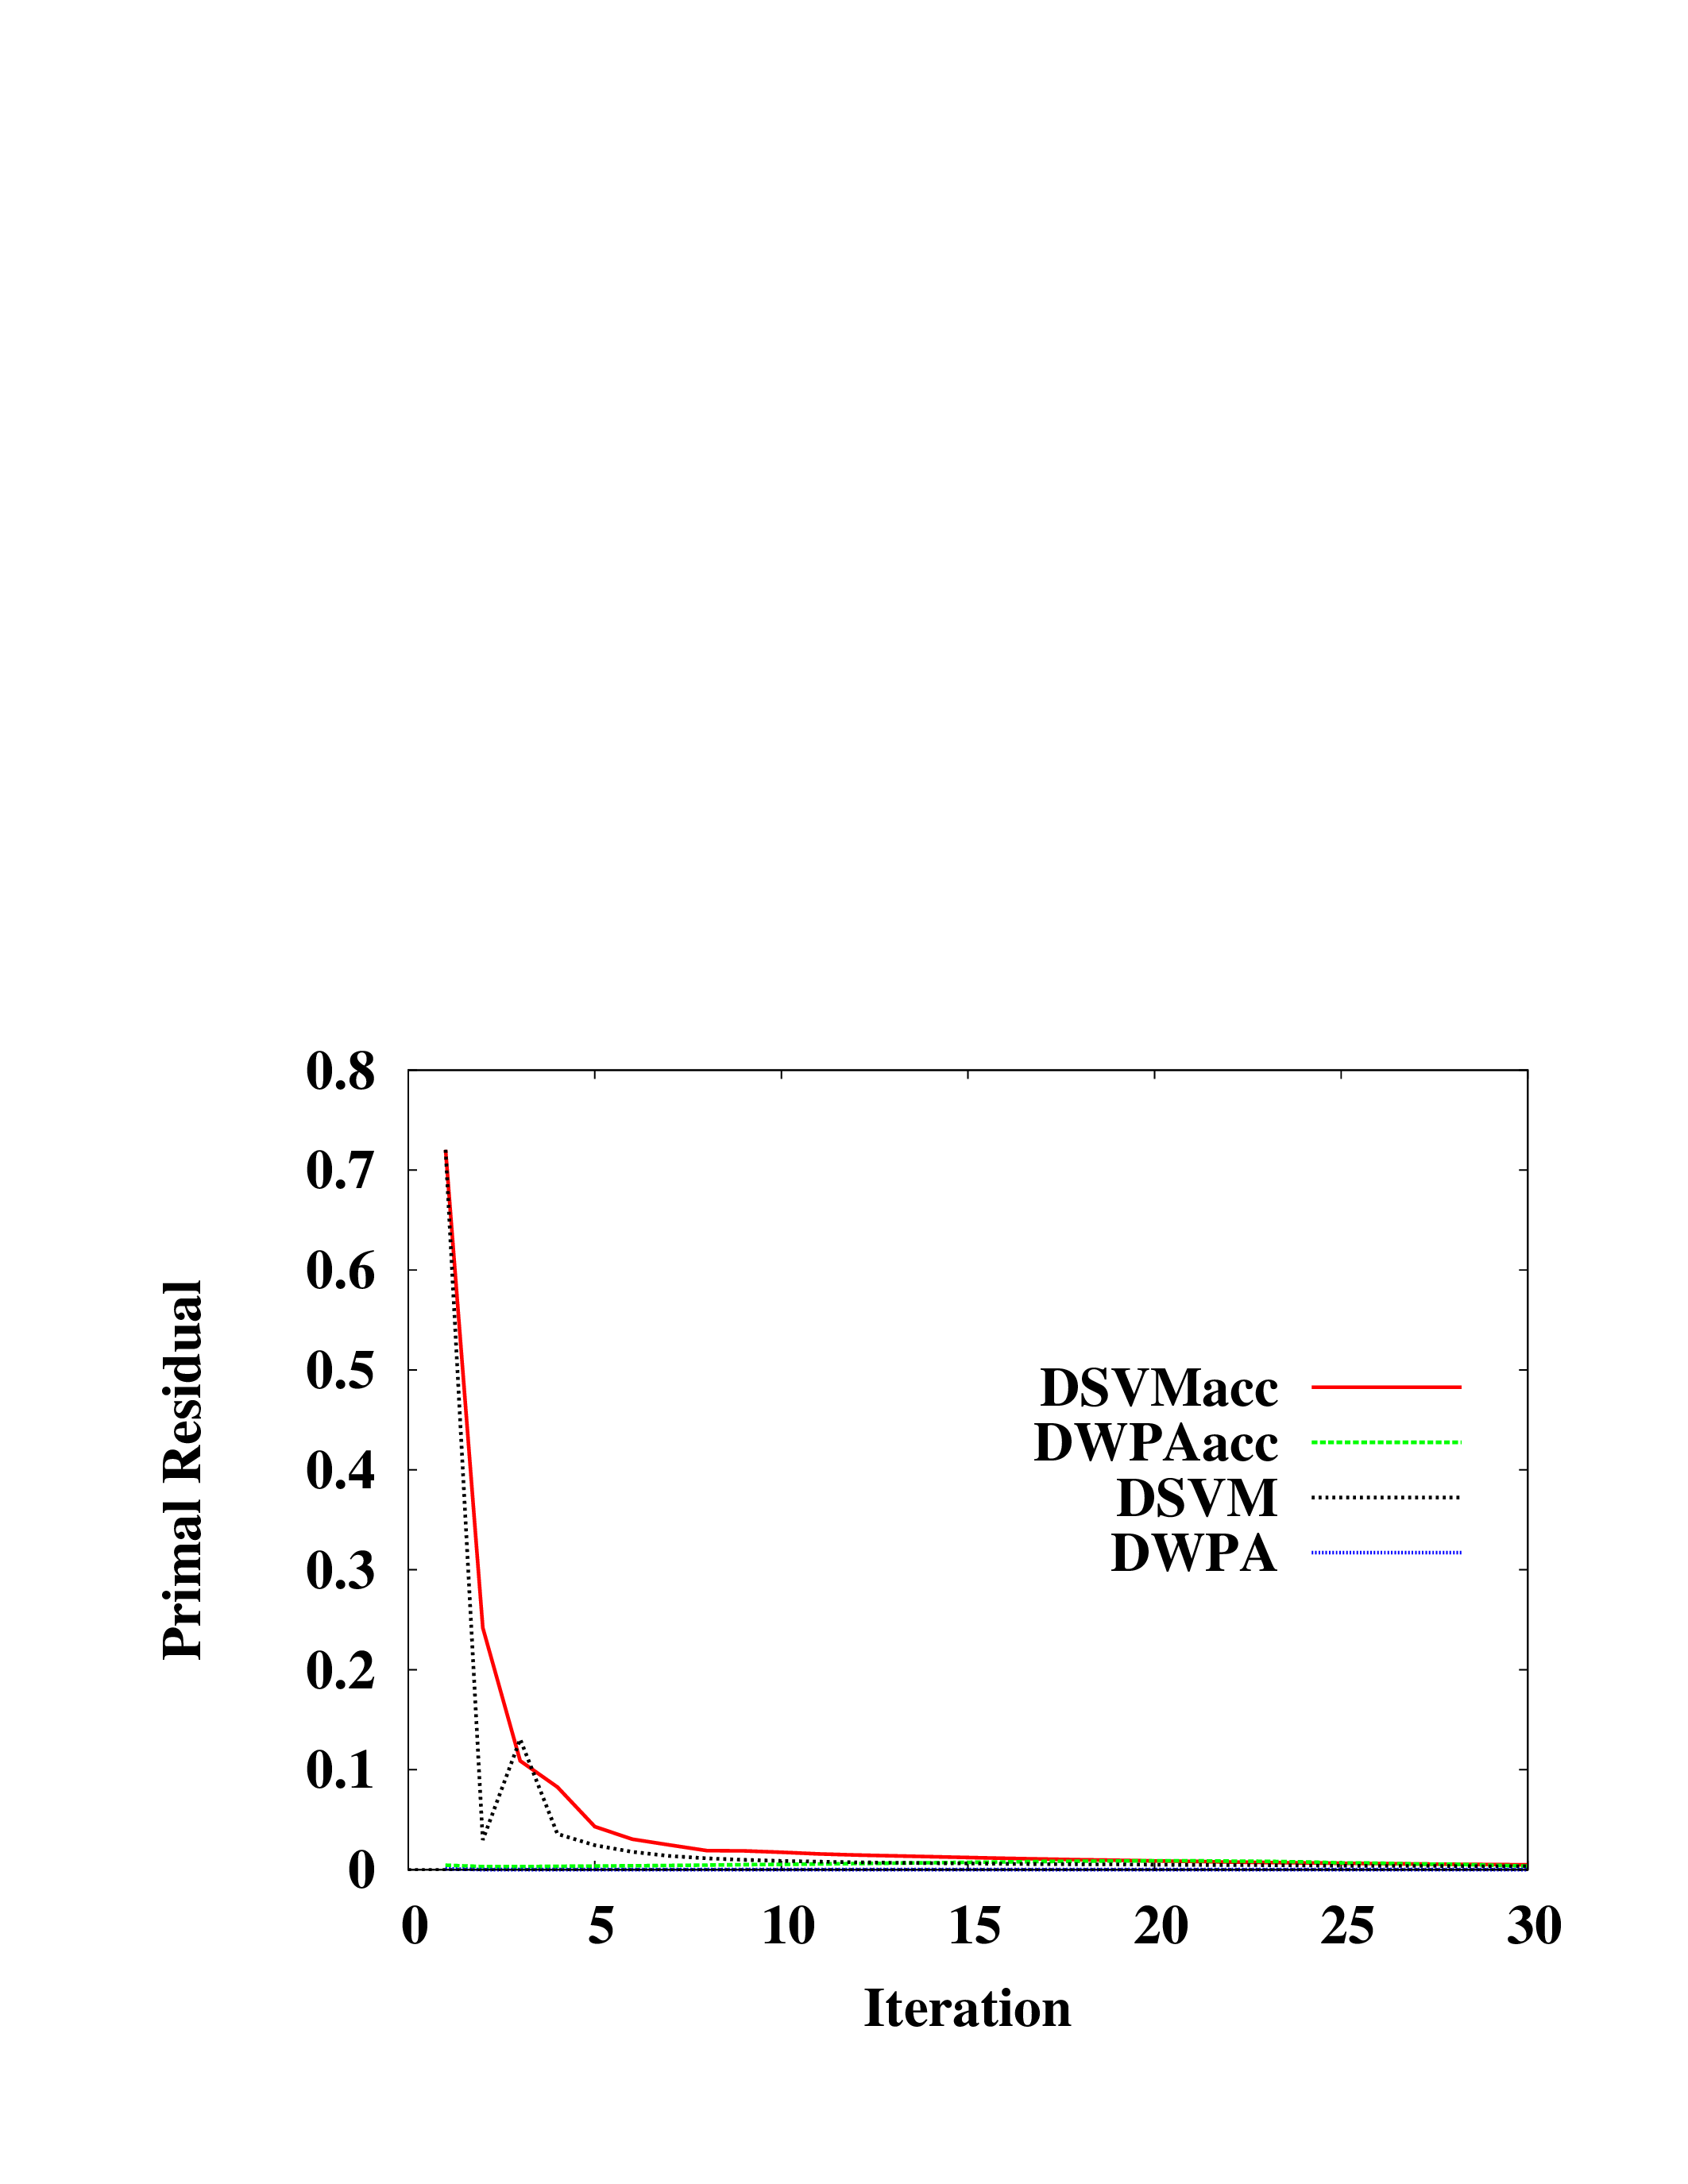}
    }
    \hspace{-.45cm}
   \subfloat[][50 partitions]{%[10 partitions]
   \includegraphics[width=0.34\linewidth]{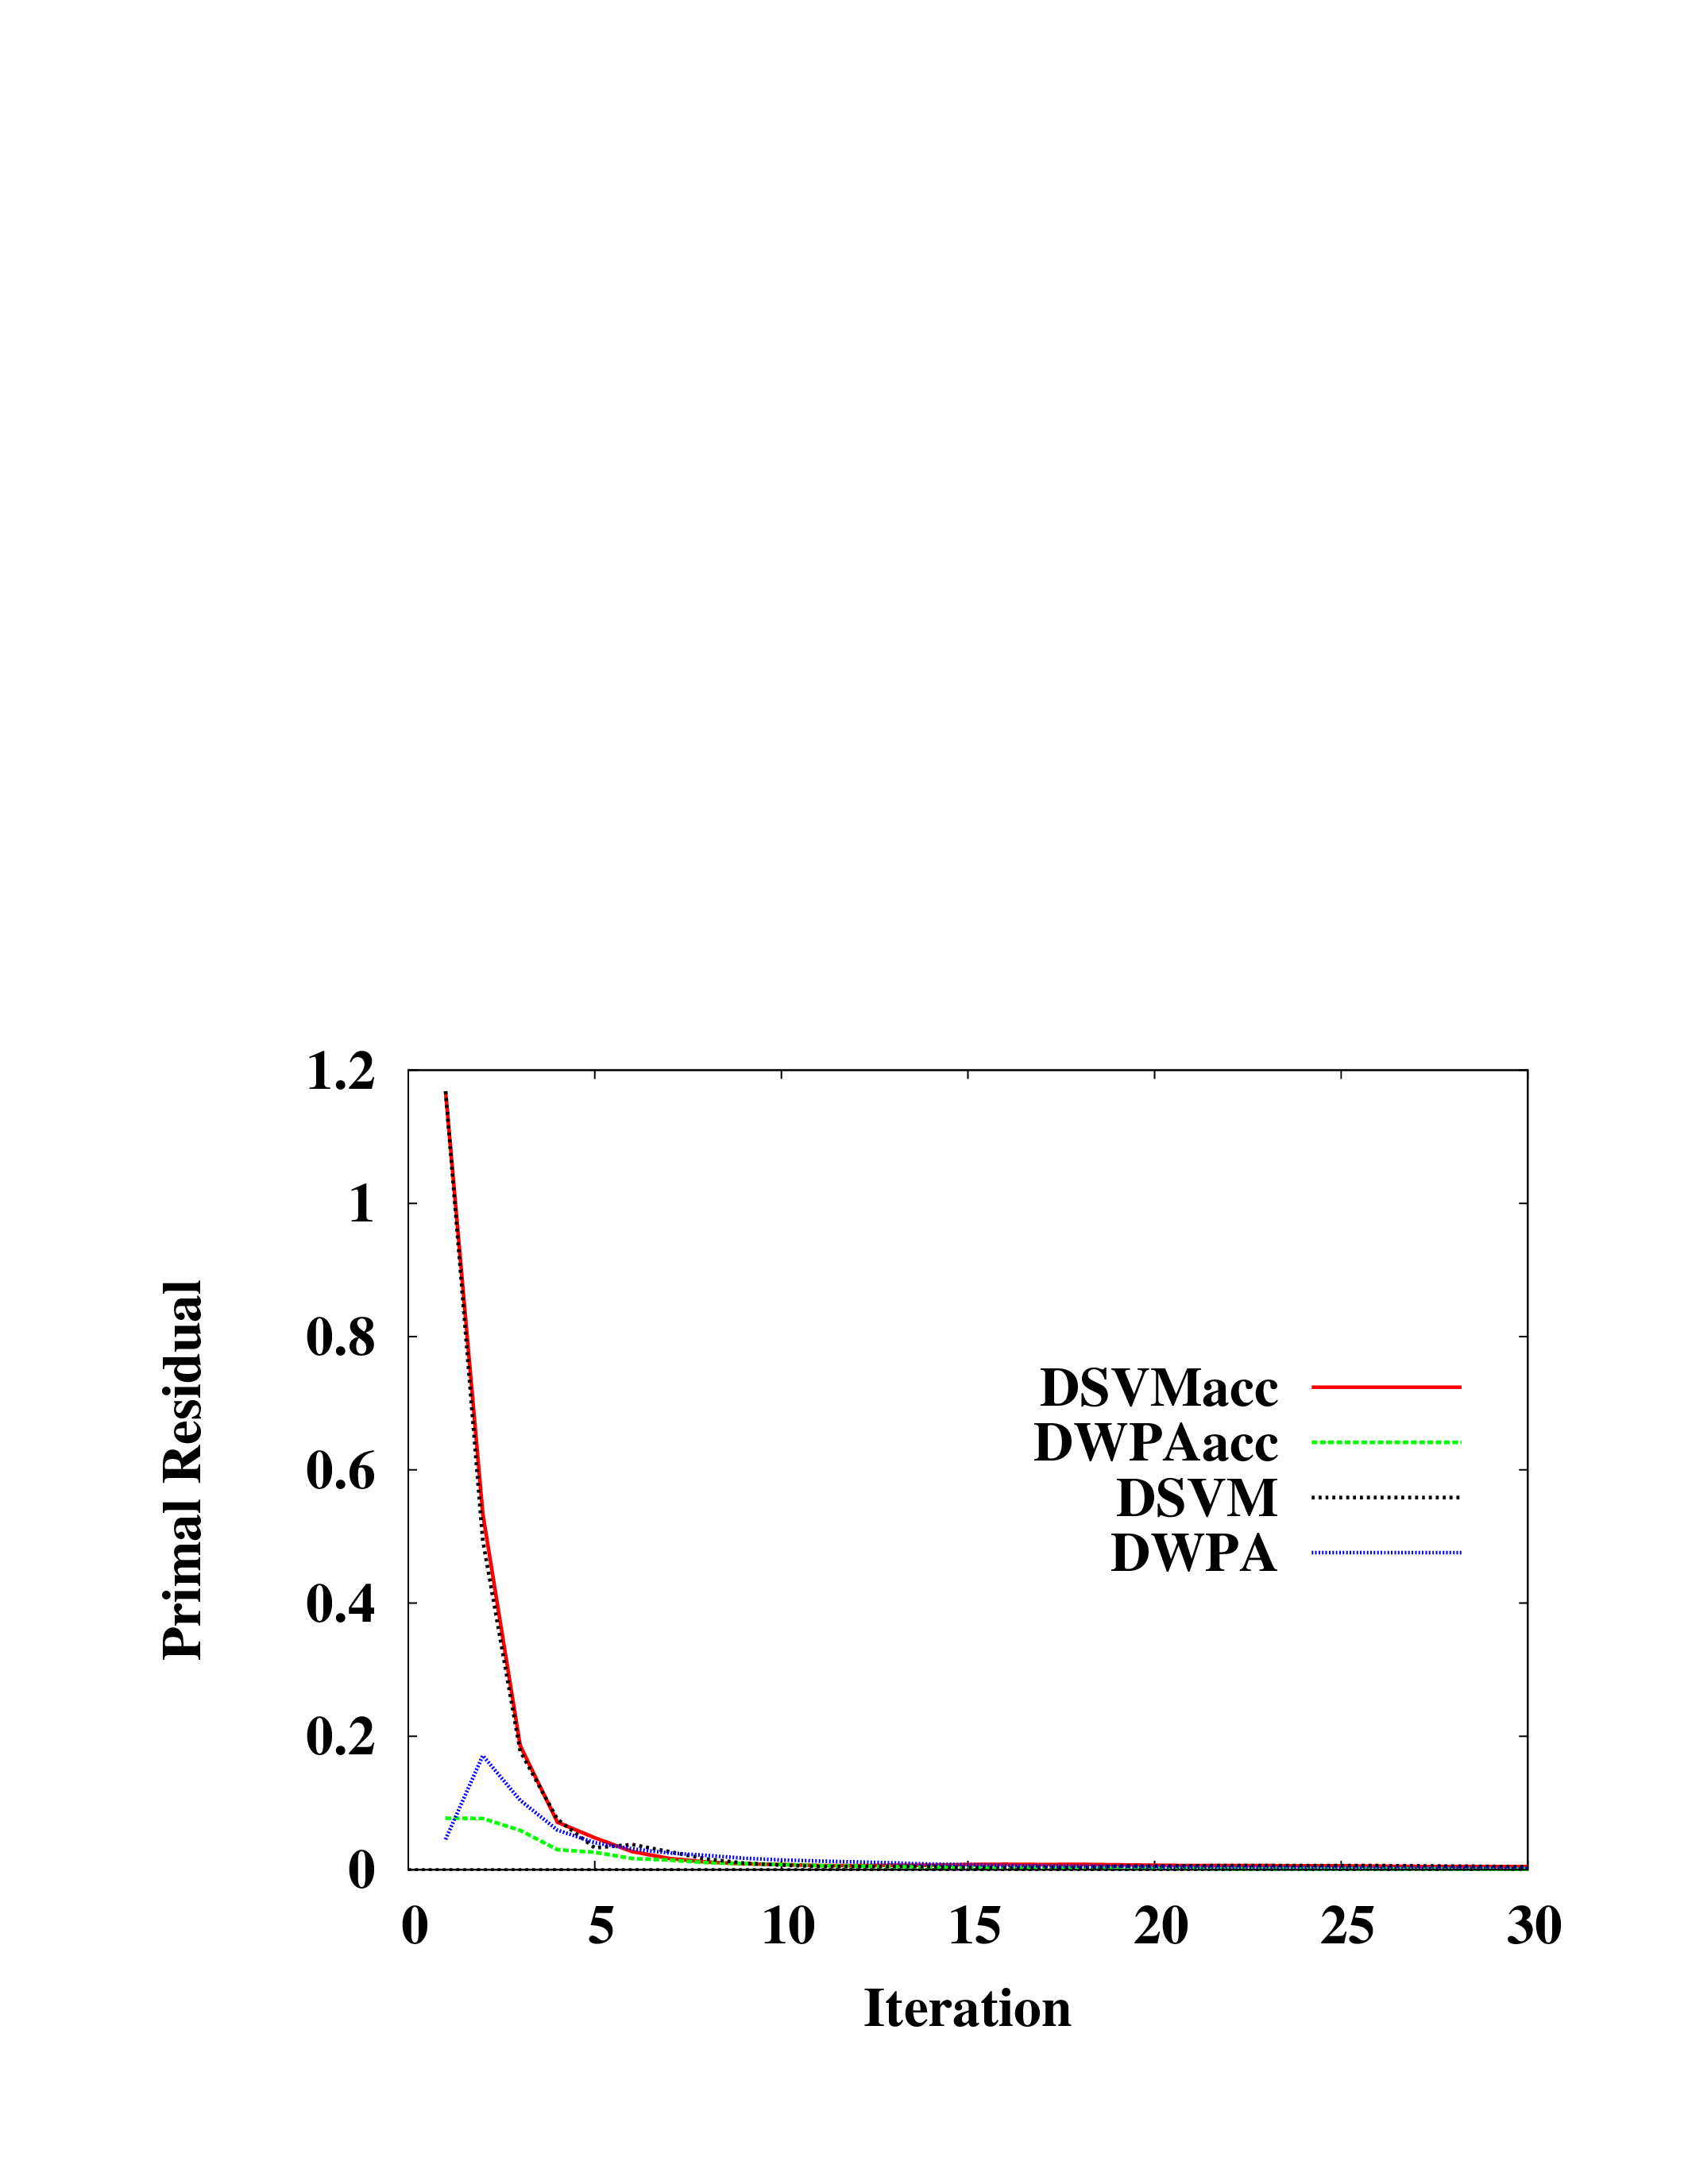}
    }
   \hspace{-.45cm}
    \subfloat[][100 partitions]{%[10 partitions]
   \includegraphics[width=0.34\linewidth]{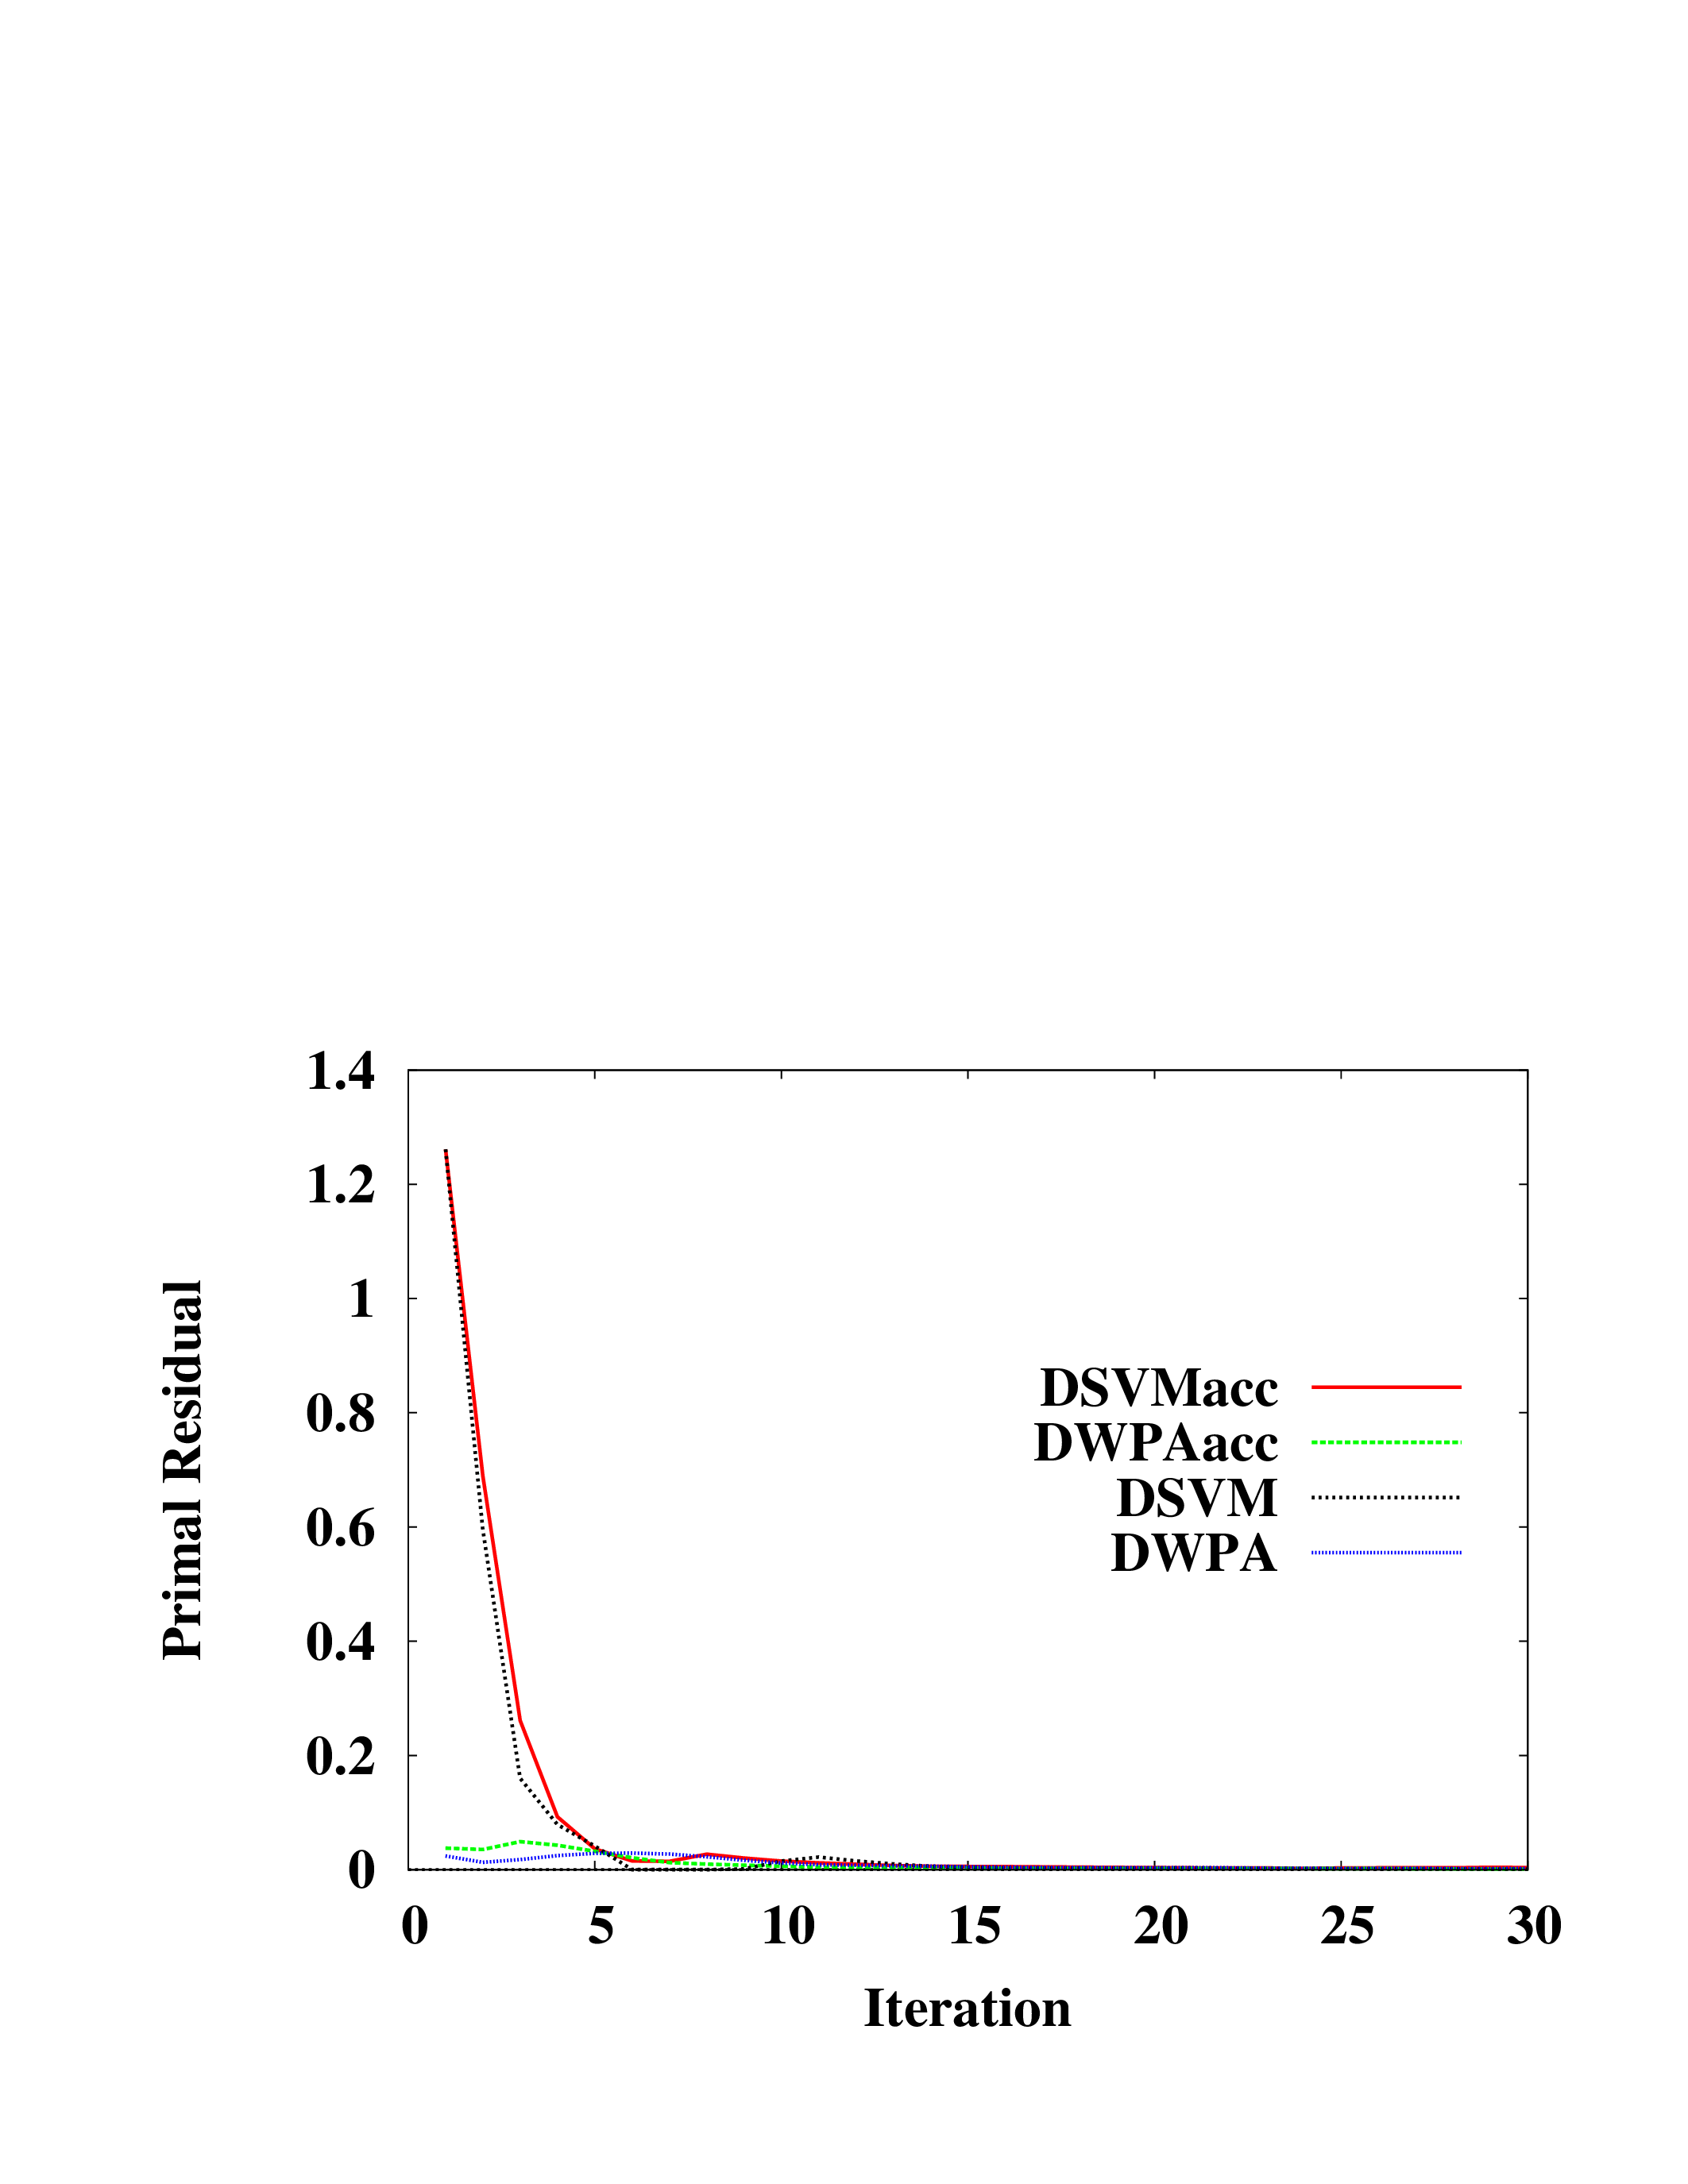}
    }
  \hspace{-.45cm}
    \subfloat[][200 partitions]{%[10 partitions]
   \includegraphics[width=0.34\linewidth]{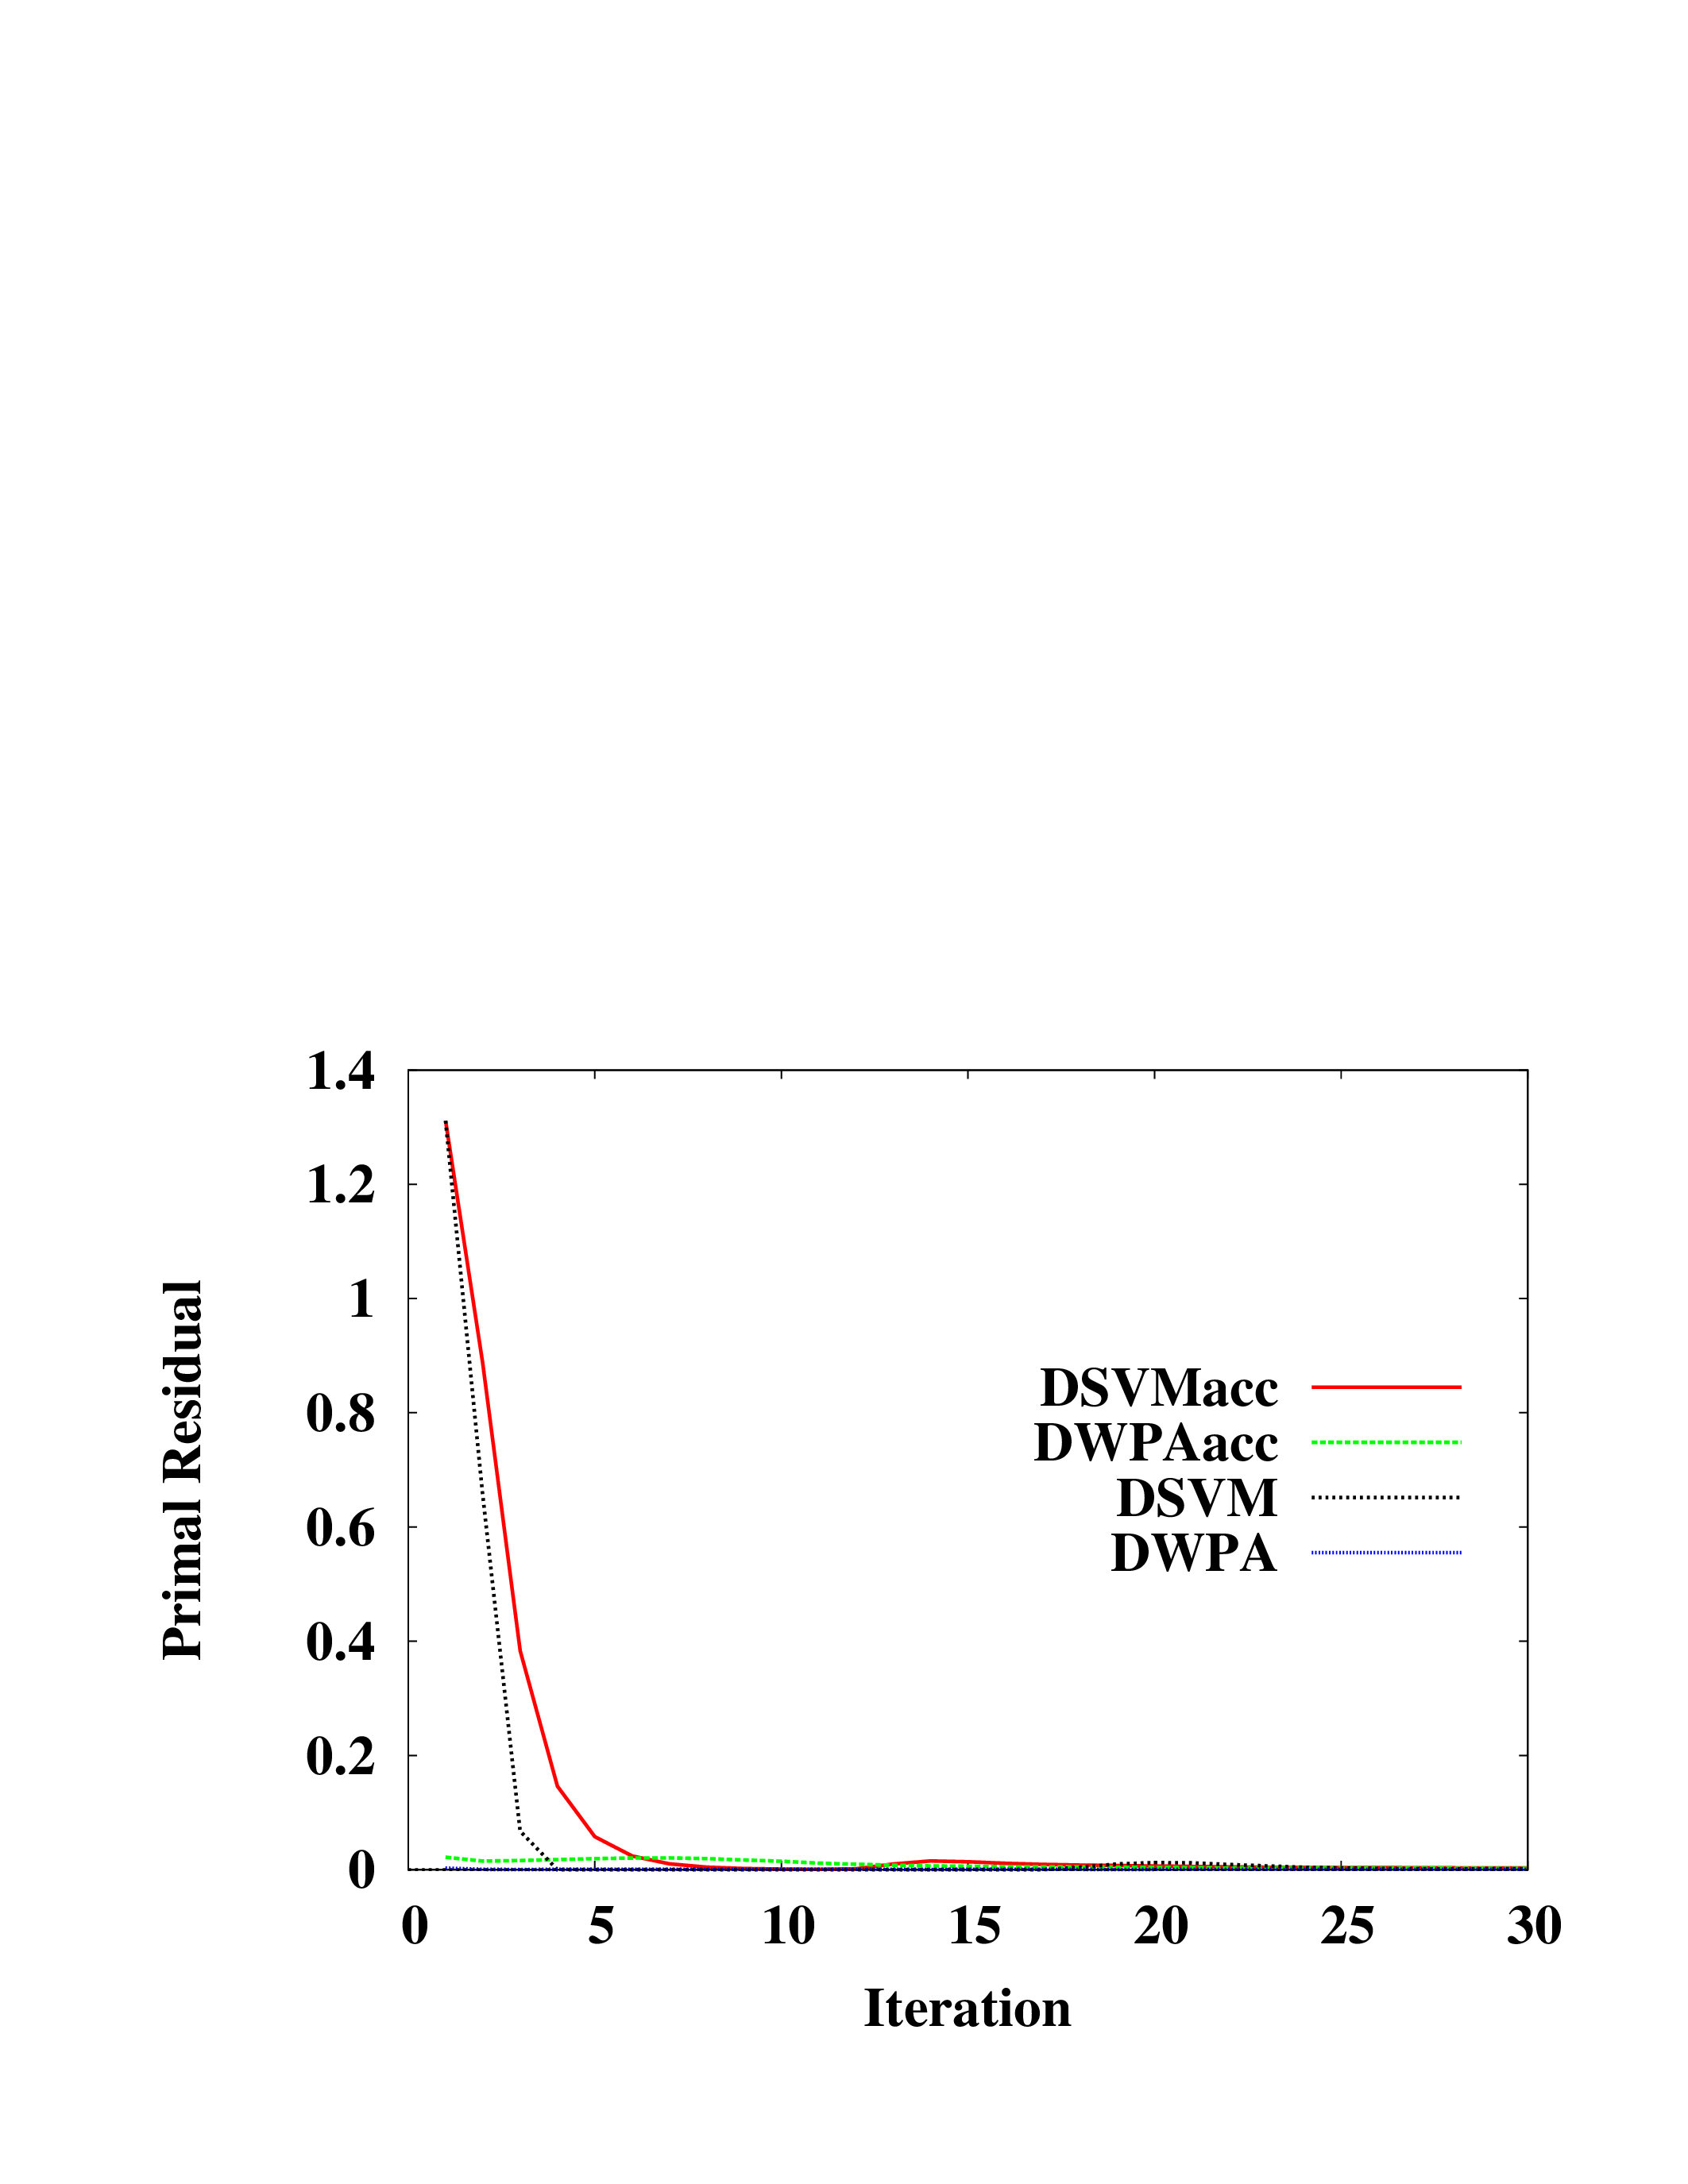}
   }
  \hspace{-.45cm}
   \subfloat[][50 partitions]{%[10 partitions]
   \includegraphics[width=0.34\linewidth]{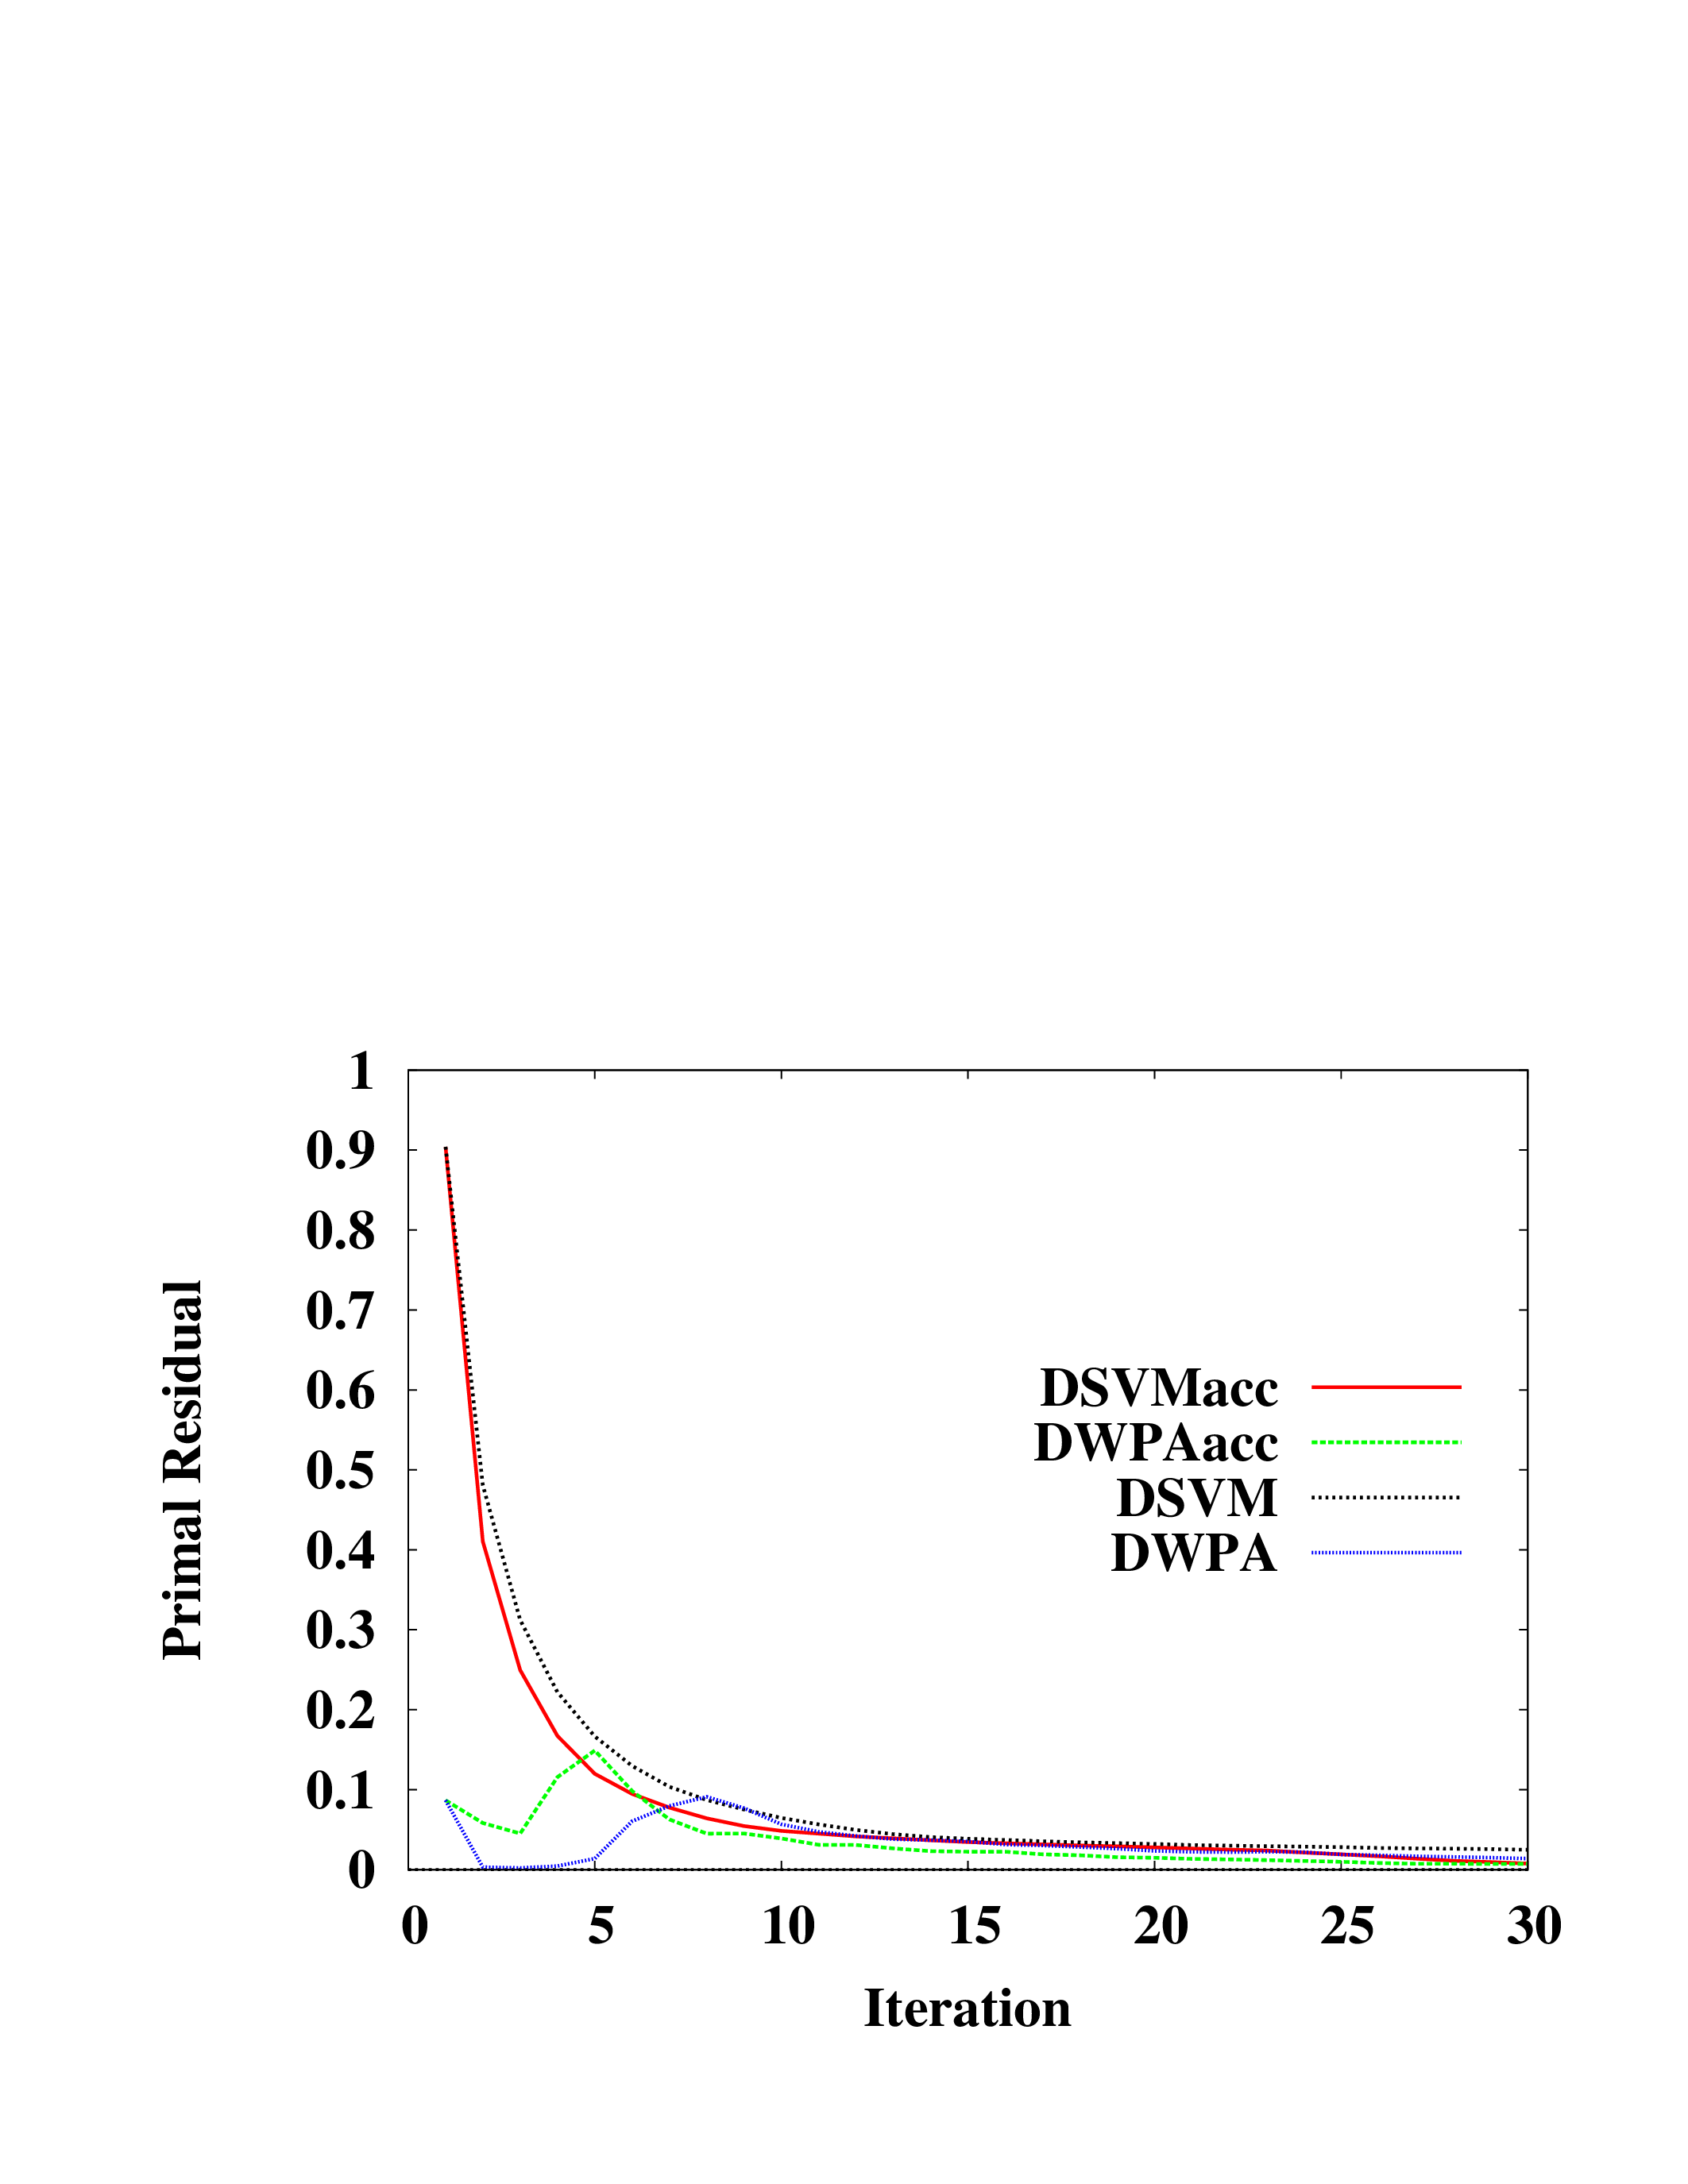}
    }
   \hspace{-.45cm}
    \subfloat[][100 partitions]{%[10 partitions]
   \includegraphics[width=0.34\linewidth]{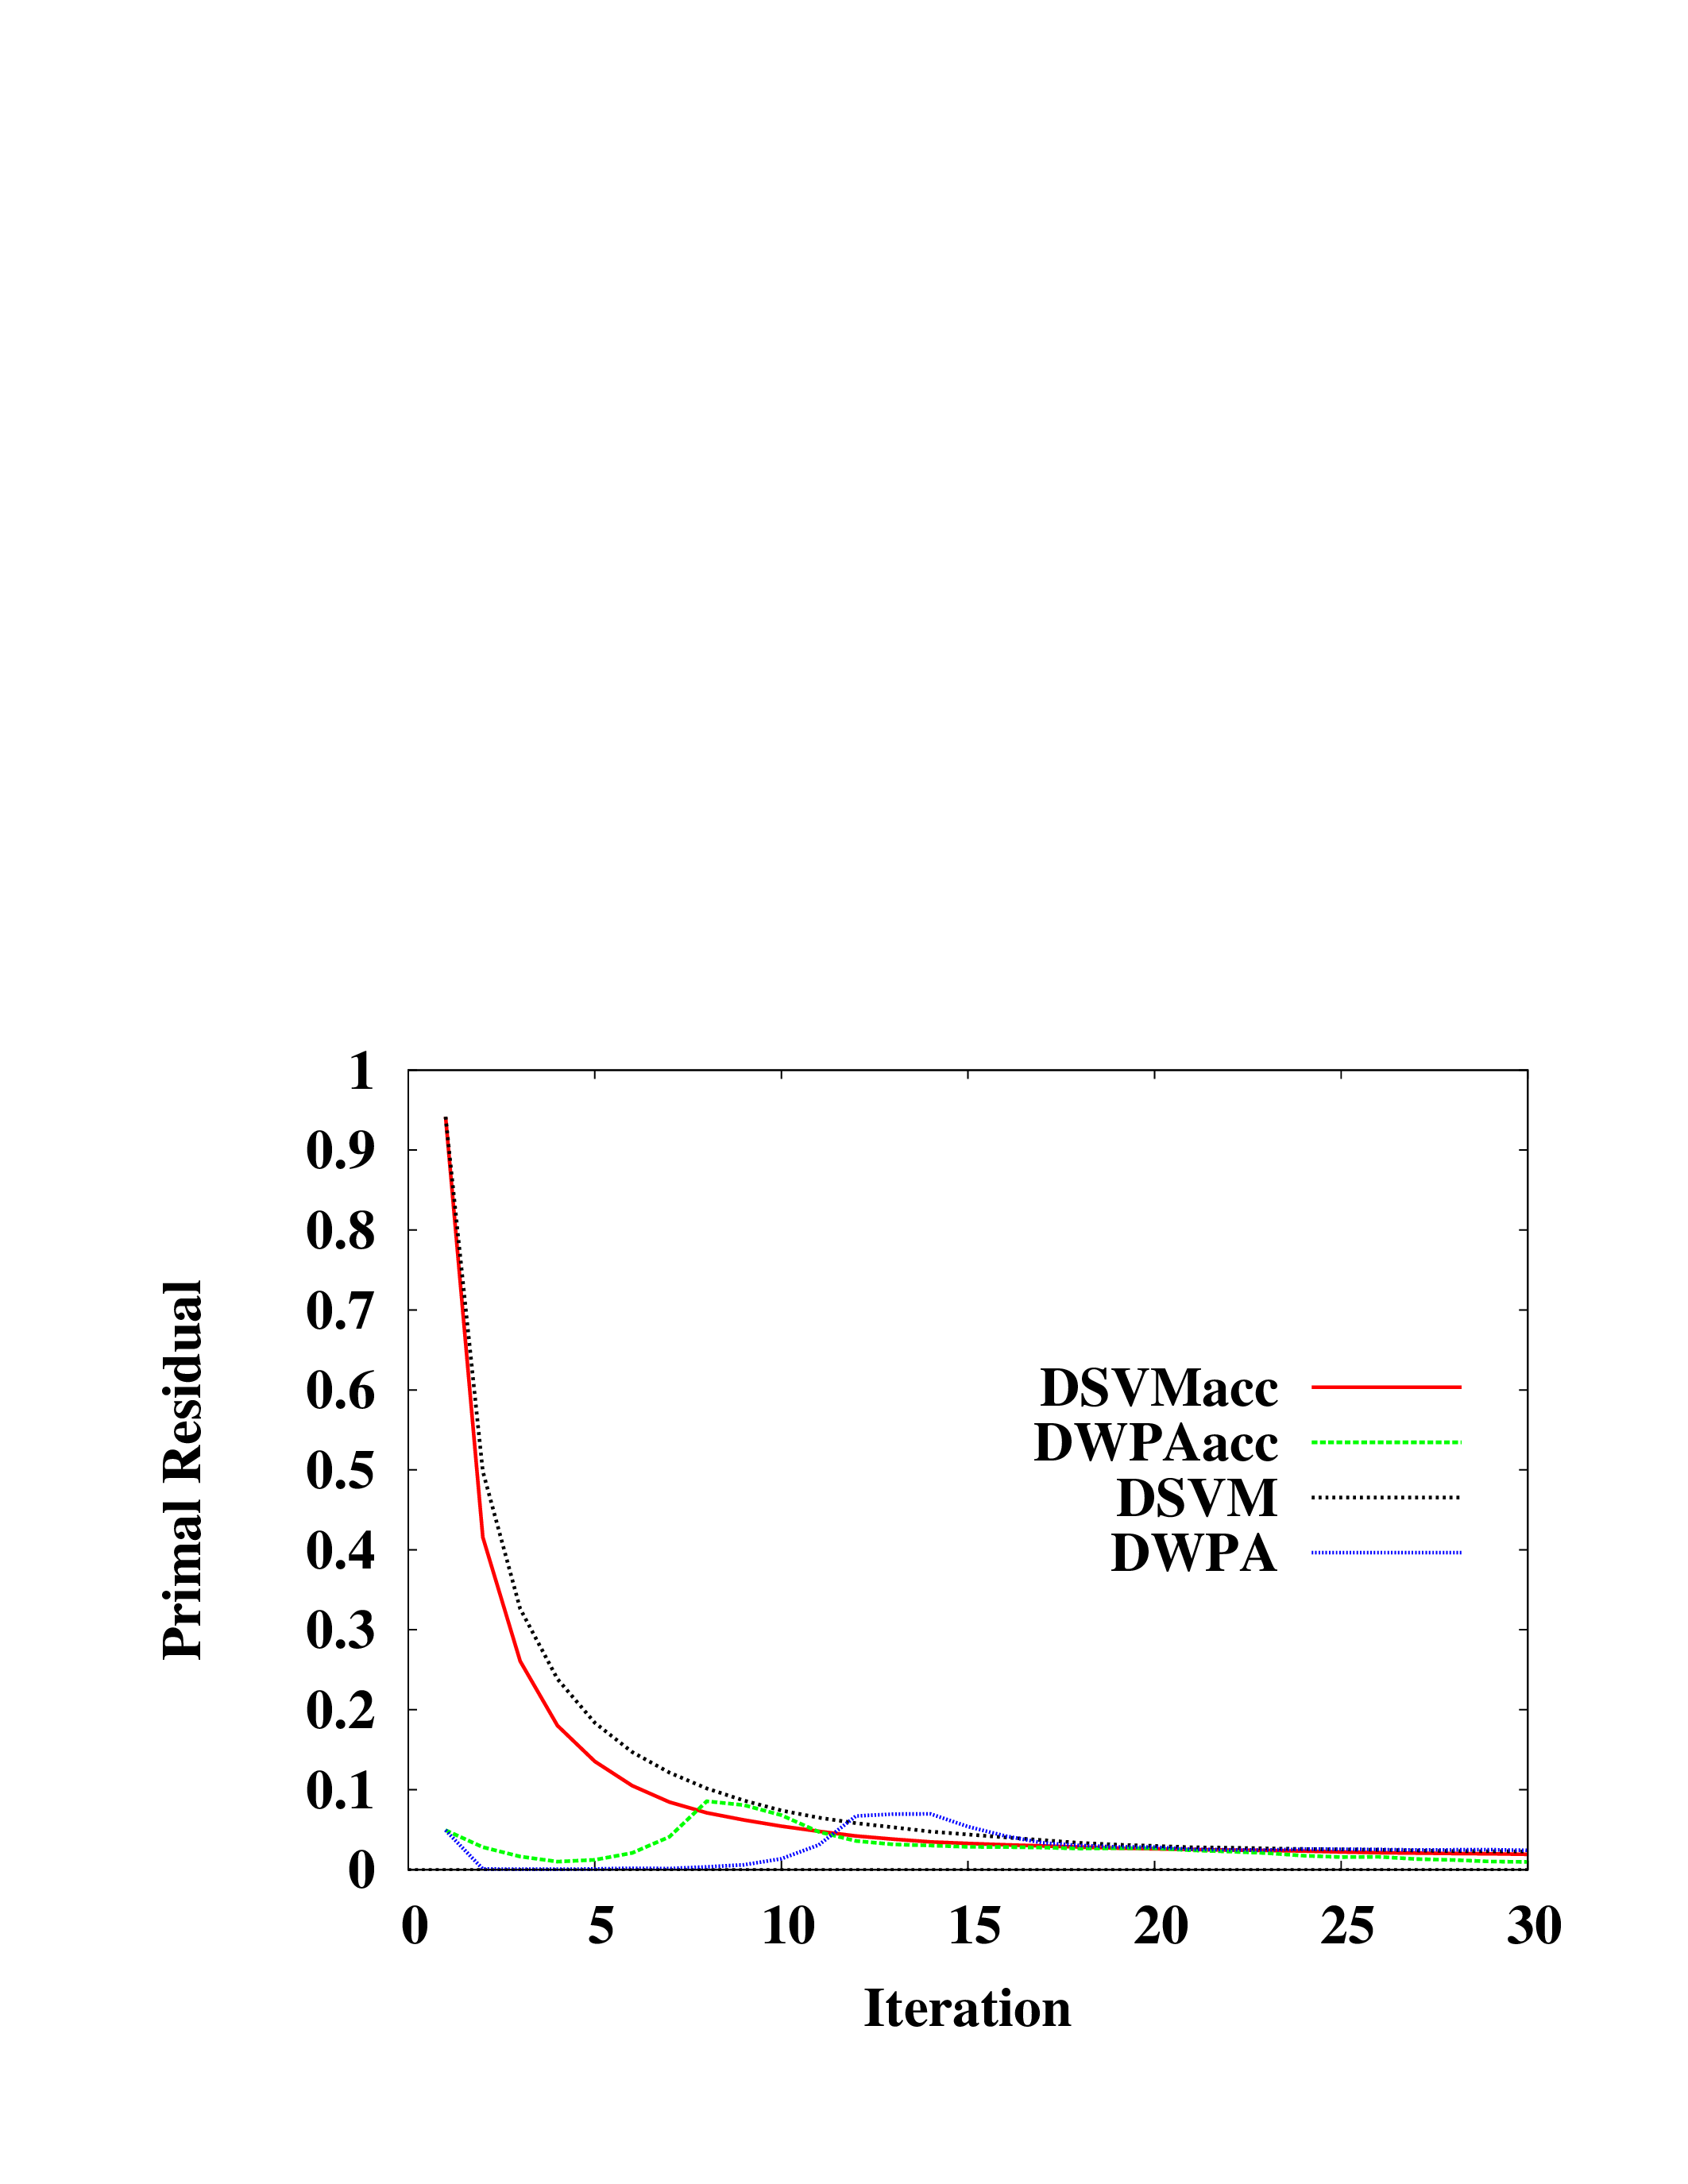}
    }
  \hspace{-.45cm}
    \subfloat[][200 partitions]{%[10 partitions]
   \includegraphics[width=0.34\linewidth]{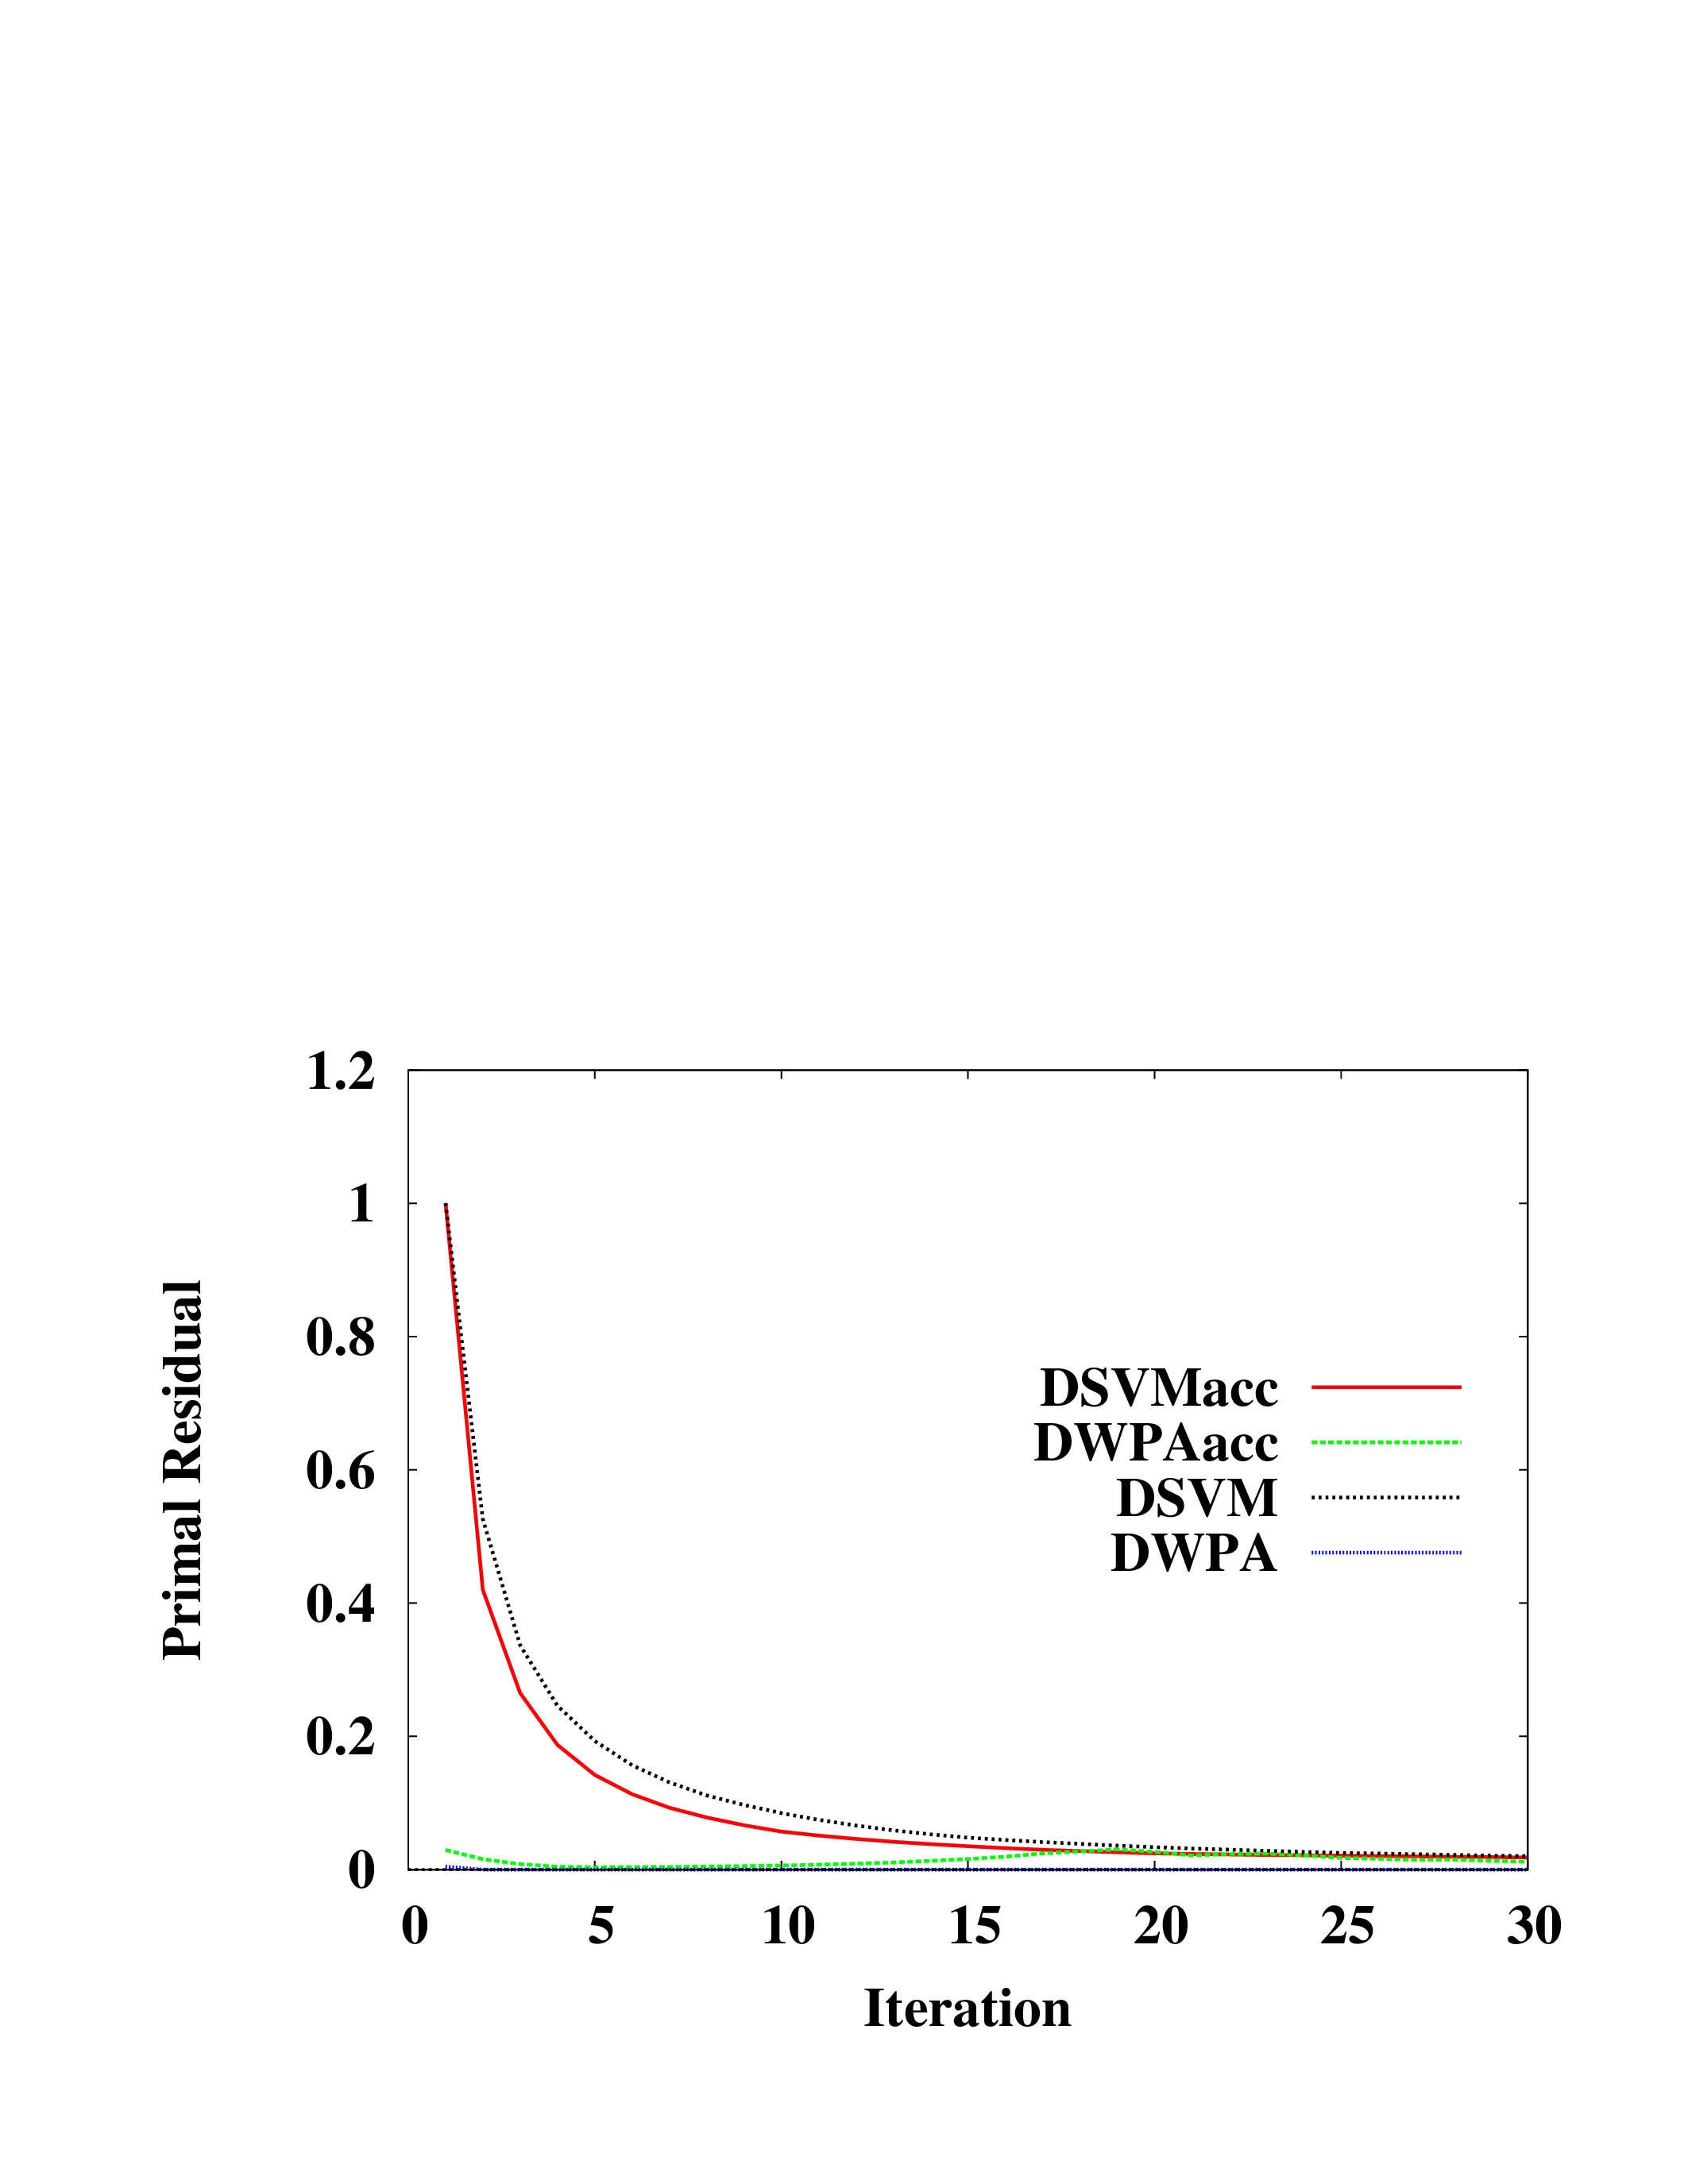}
   }   
 \end{center}
 %\vspace{-0.8cm}
   \caption{\label{pe}Convergence of primal residual for \textbf{real-sim}(top), \textbf{epsilon}(middle) and \textbf{gisette}(bottom)}
%\vspace{-0.75cm}
 \end{figure}

\textbf{Convergence of testset accuracies}\\
   \begin{figure}[!ht] 
   \captionsetup[subfigure]{labelformat=empty}
  \begin{center}
   \subfloat[]{%[50 partitions]{%[10 partitions]
   \includegraphics[width=0.34\linewidth]{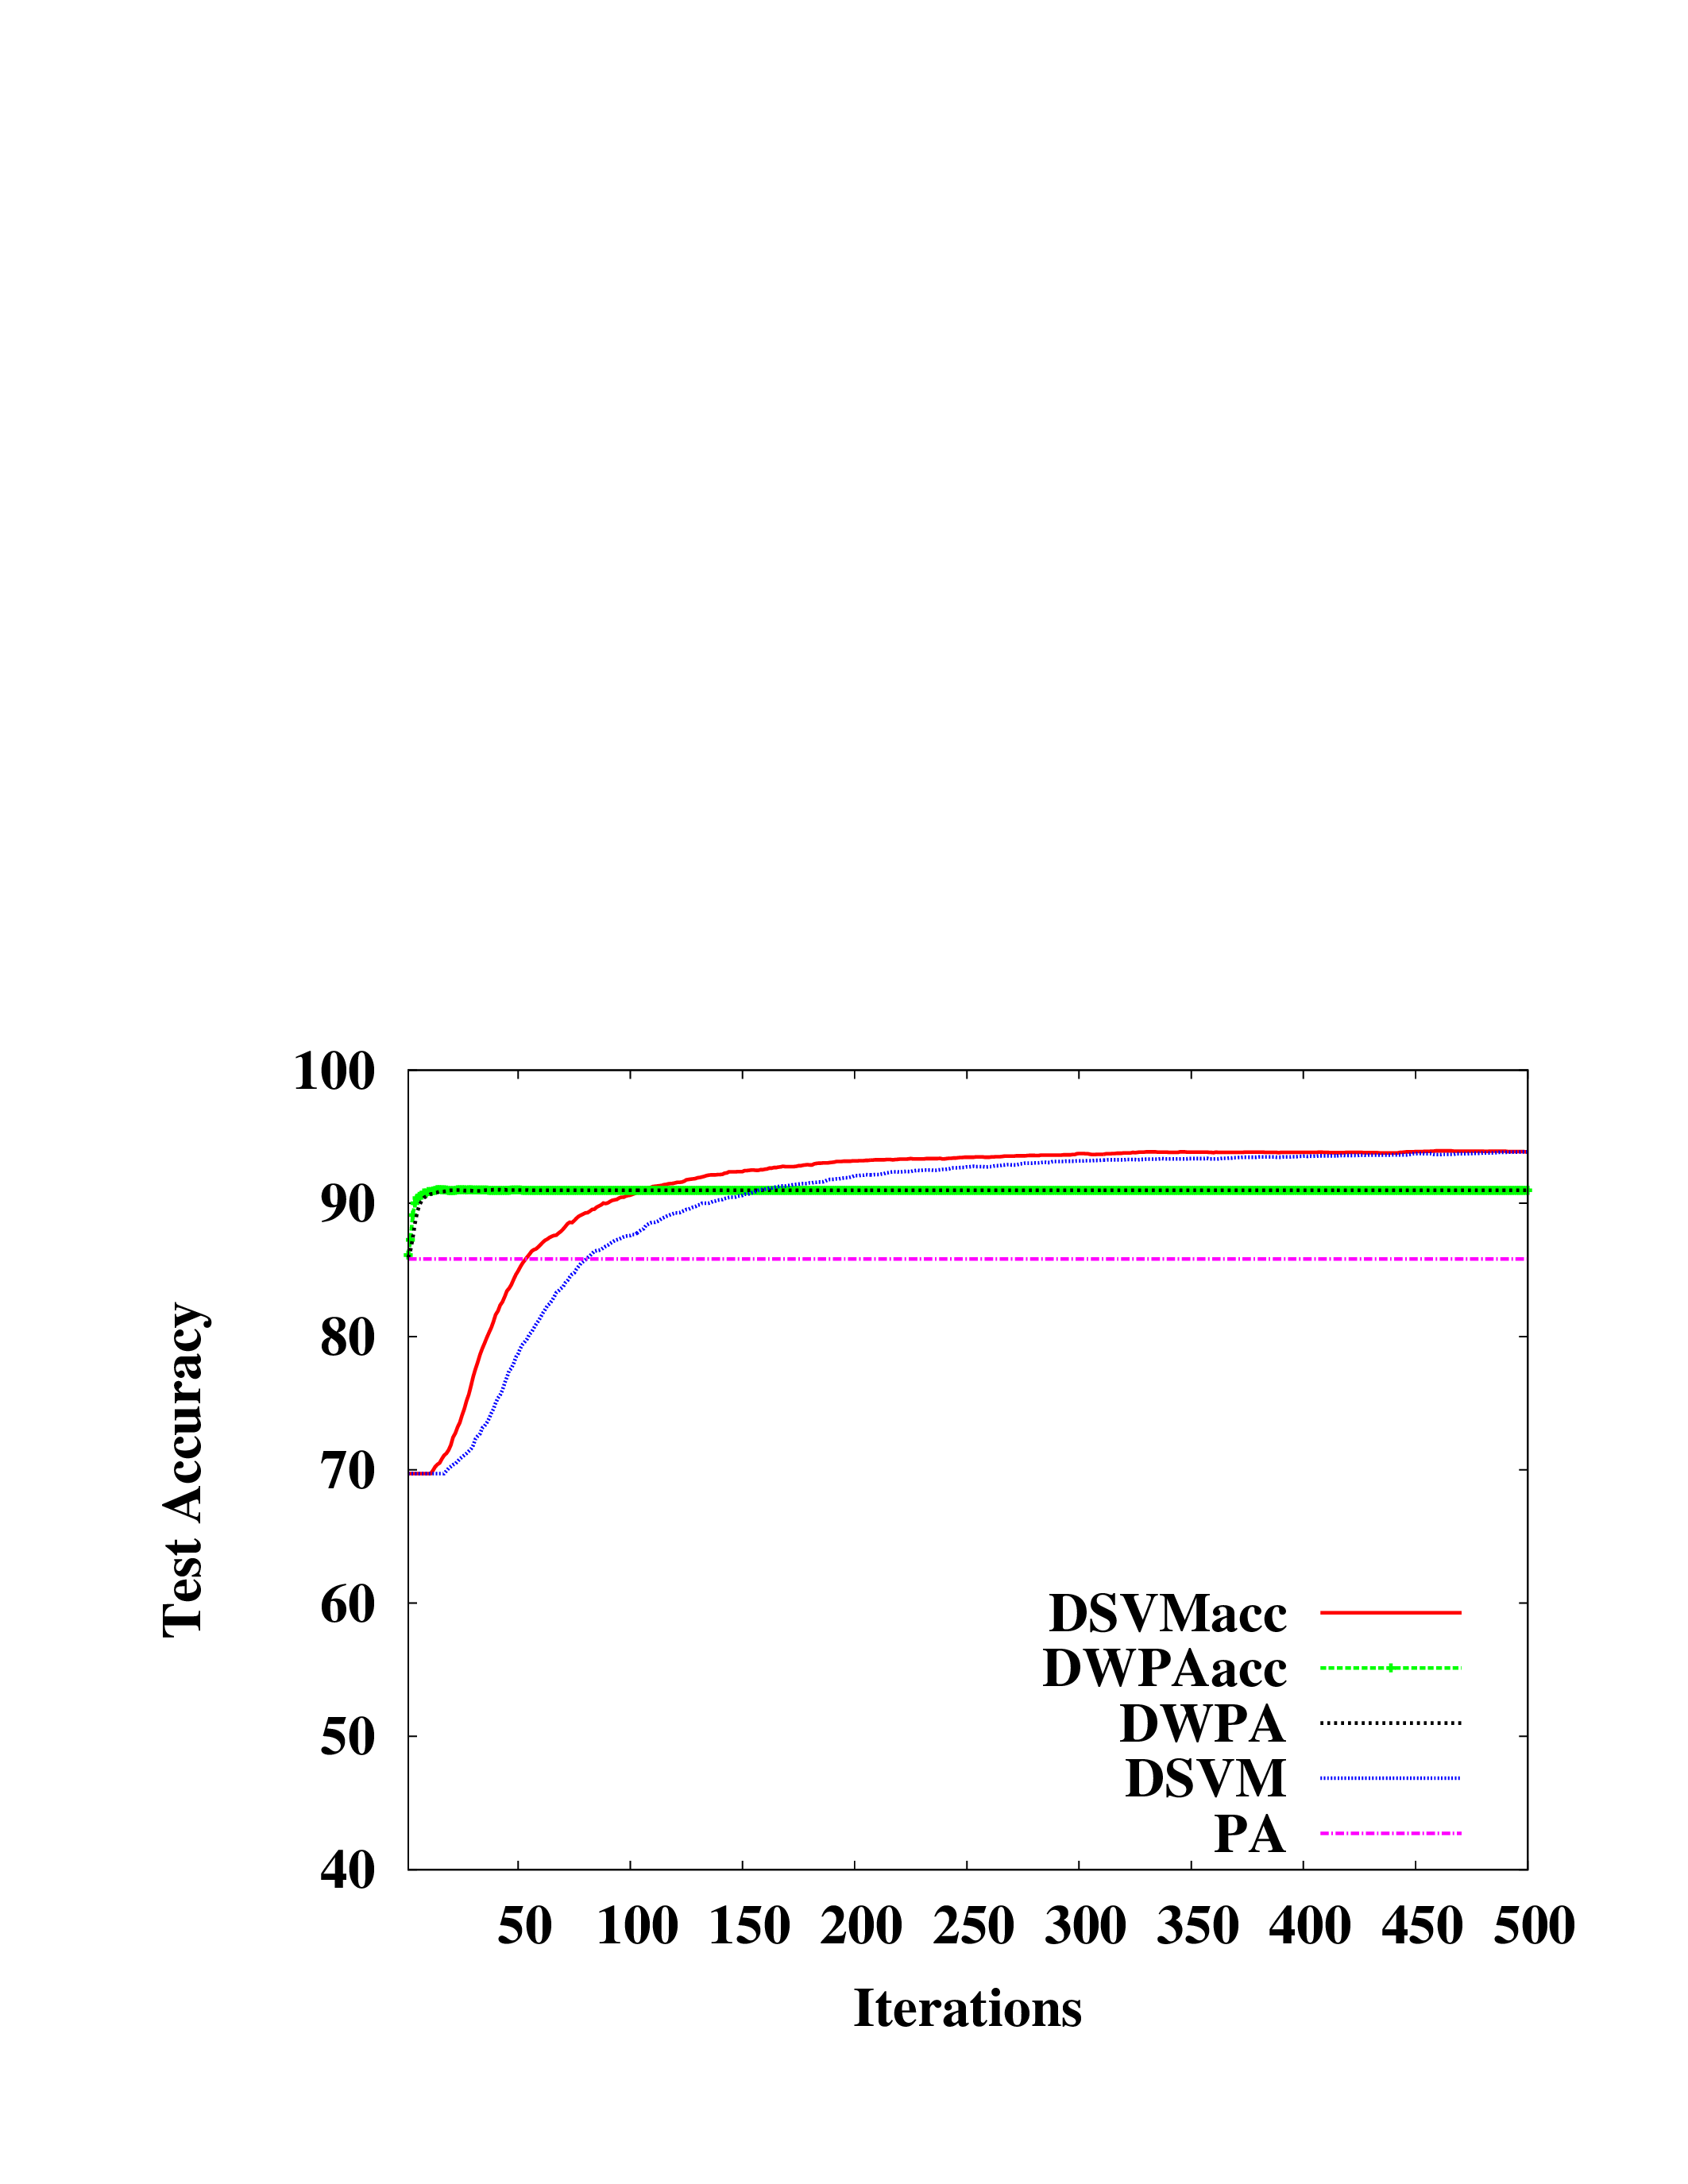}
    }
 %  \vspace{-1.6cm}
   \hspace{-.45cm}
    \subfloat[]{%[100 partitions]{%[10 partitions]
   \includegraphics[width=0.34\linewidth]{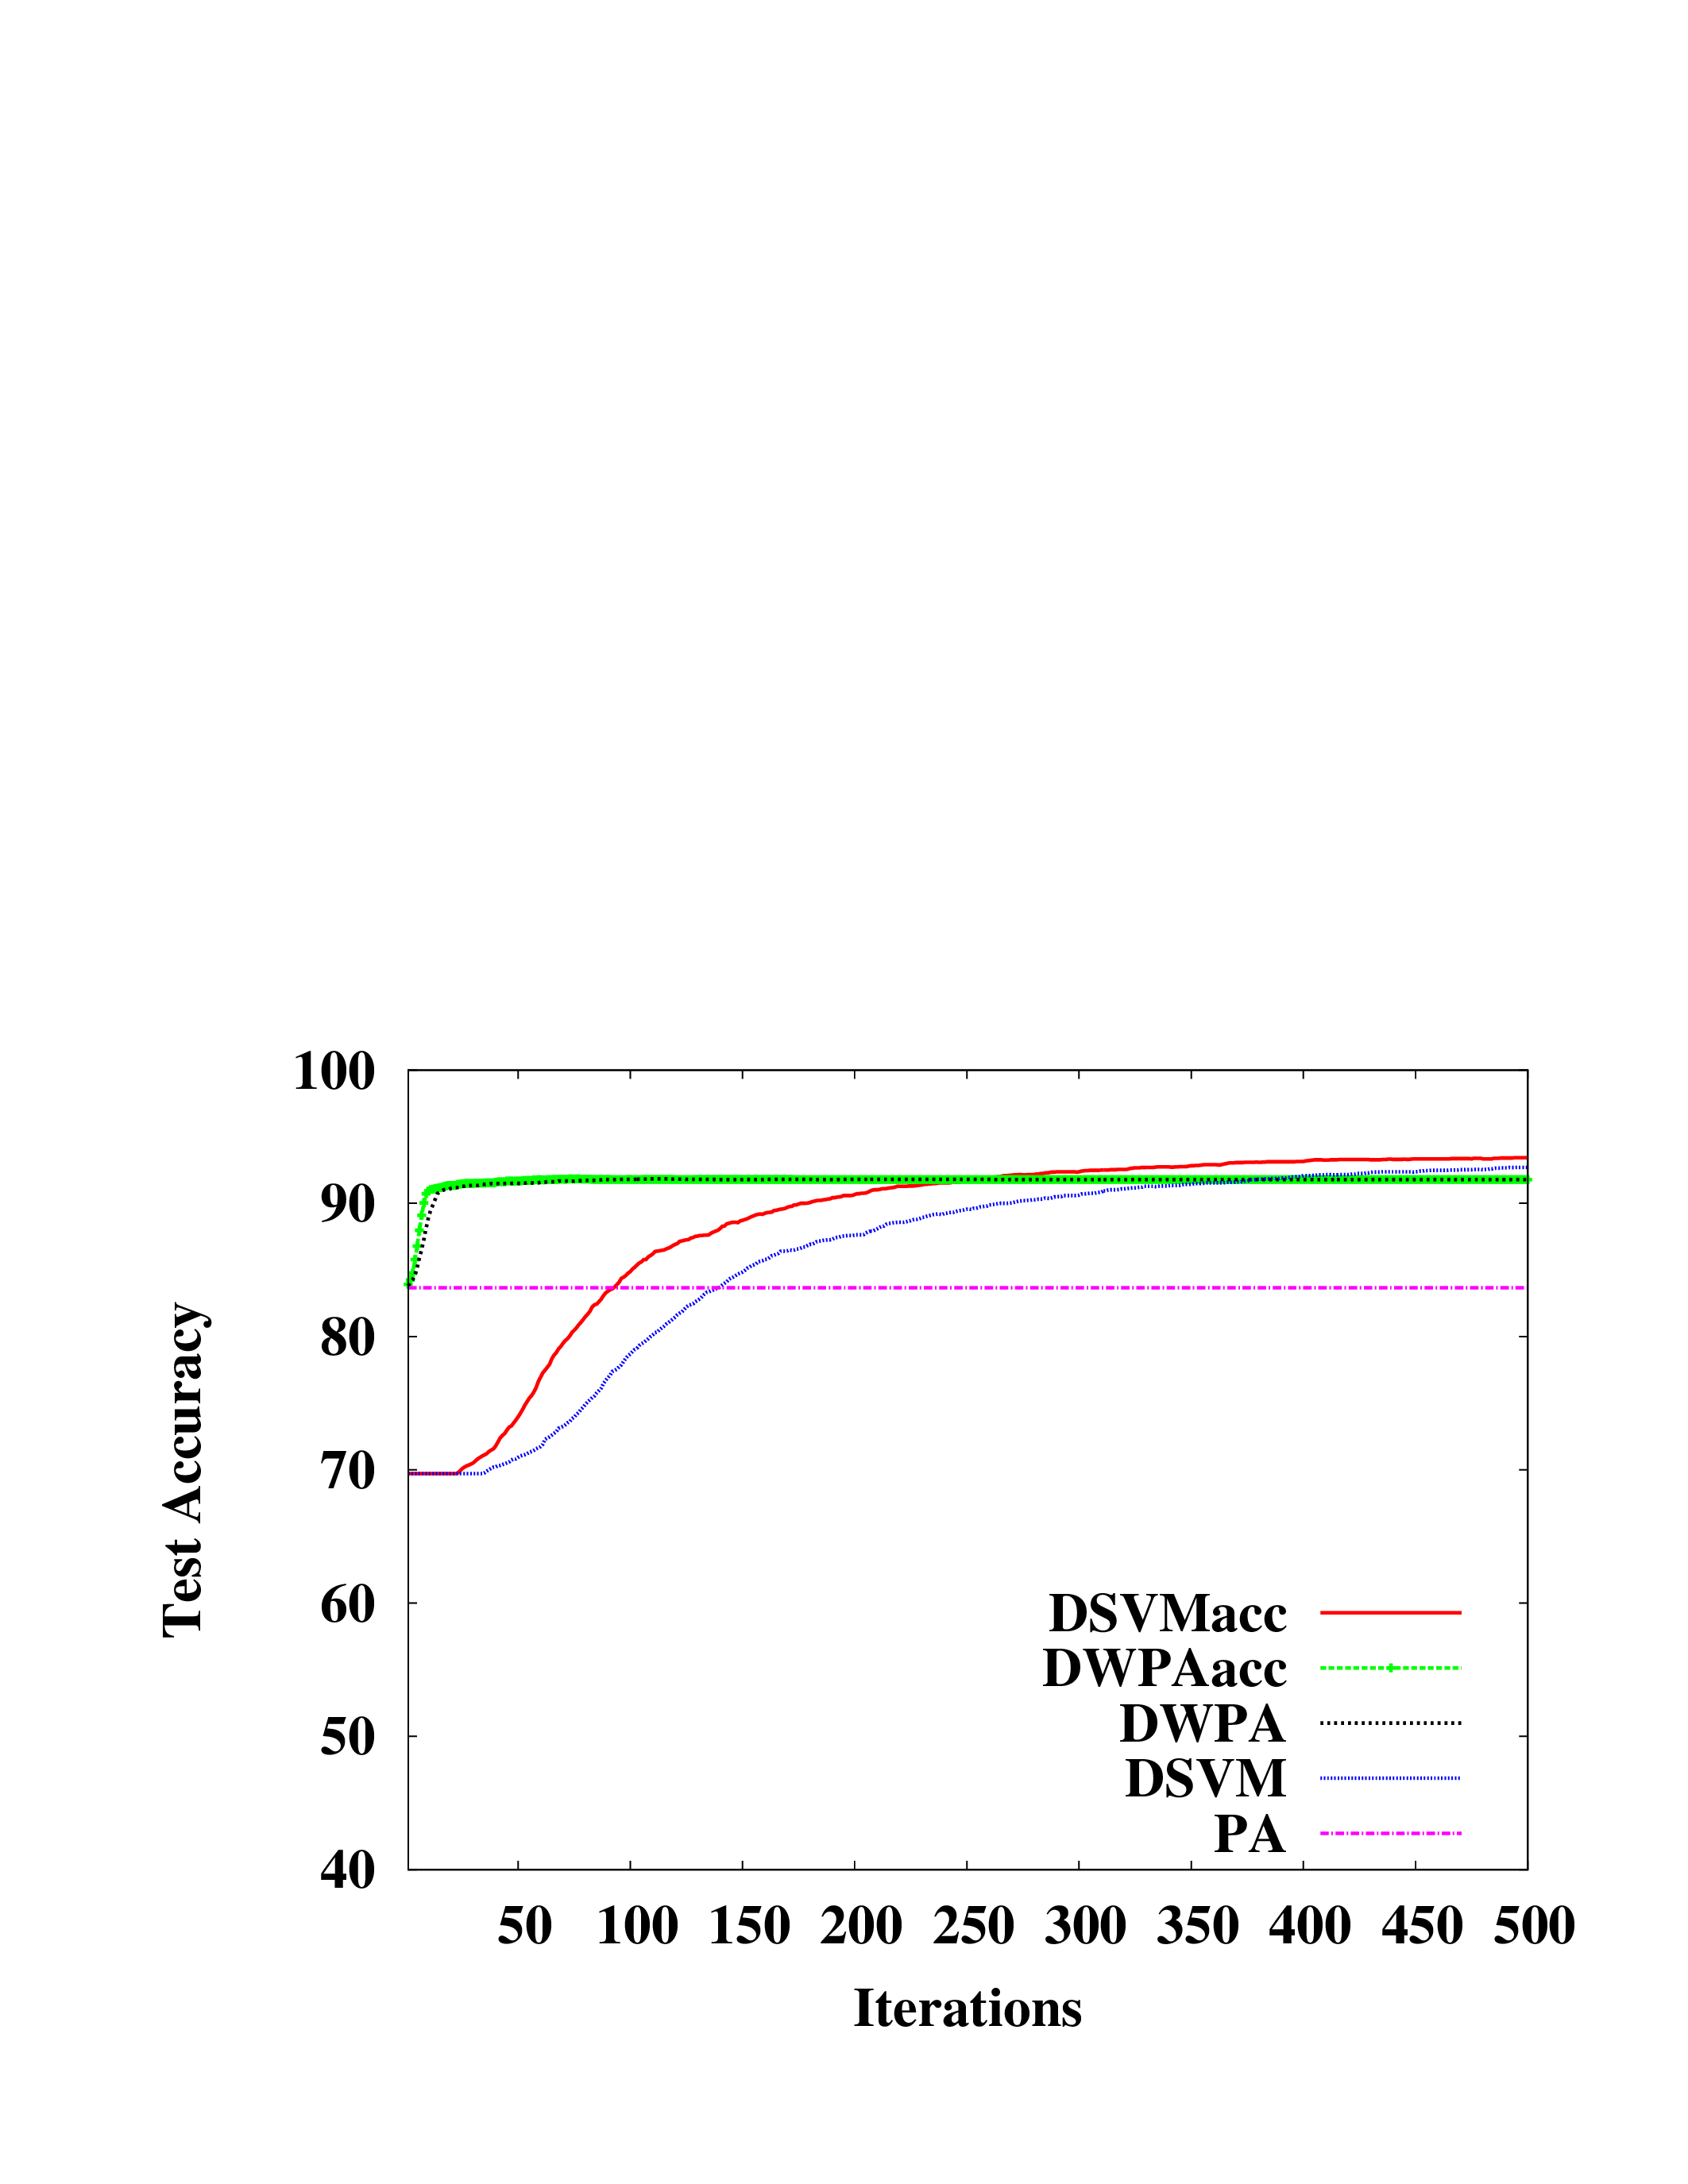}
    }
    \hspace{-.45cm}
    \subfloat[]{%[200 partitions]{%[10 partitions]
   \includegraphics[width=0.34\linewidth]{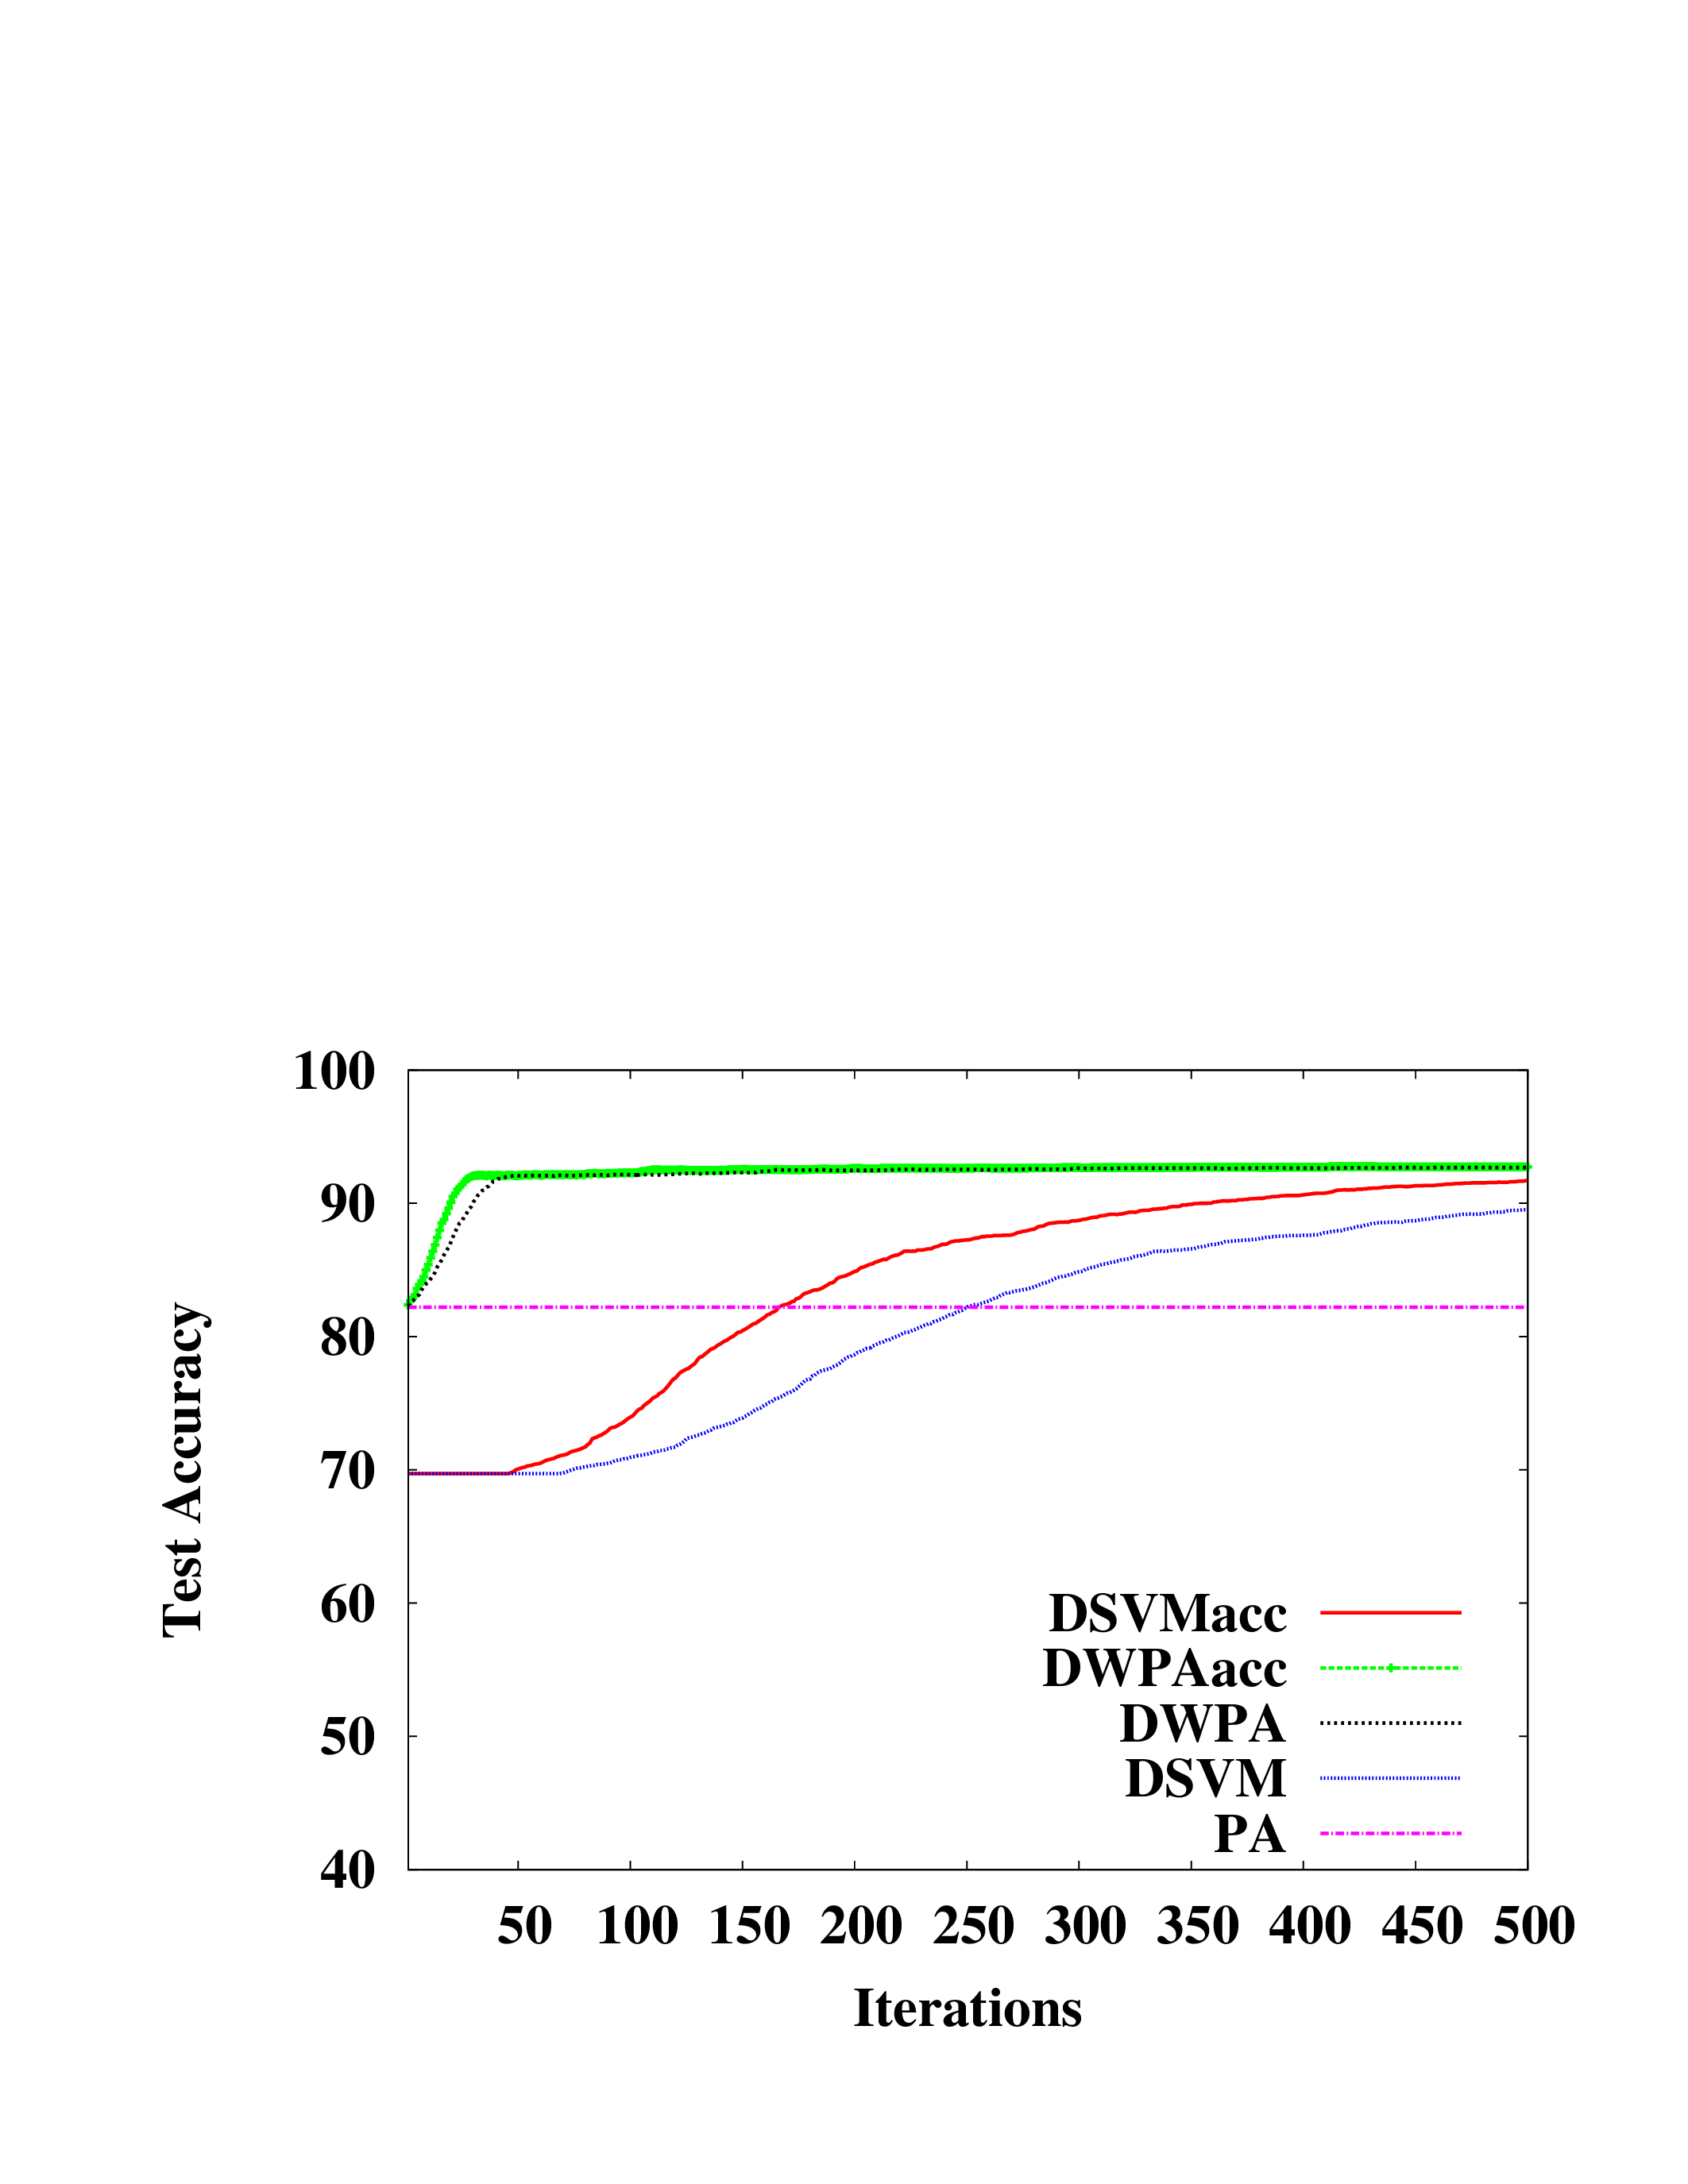}
    }
    \hspace{-.45cm}
   \subfloat[][50 partitions]{%[10 partitions]
   \includegraphics[width=0.34\linewidth]{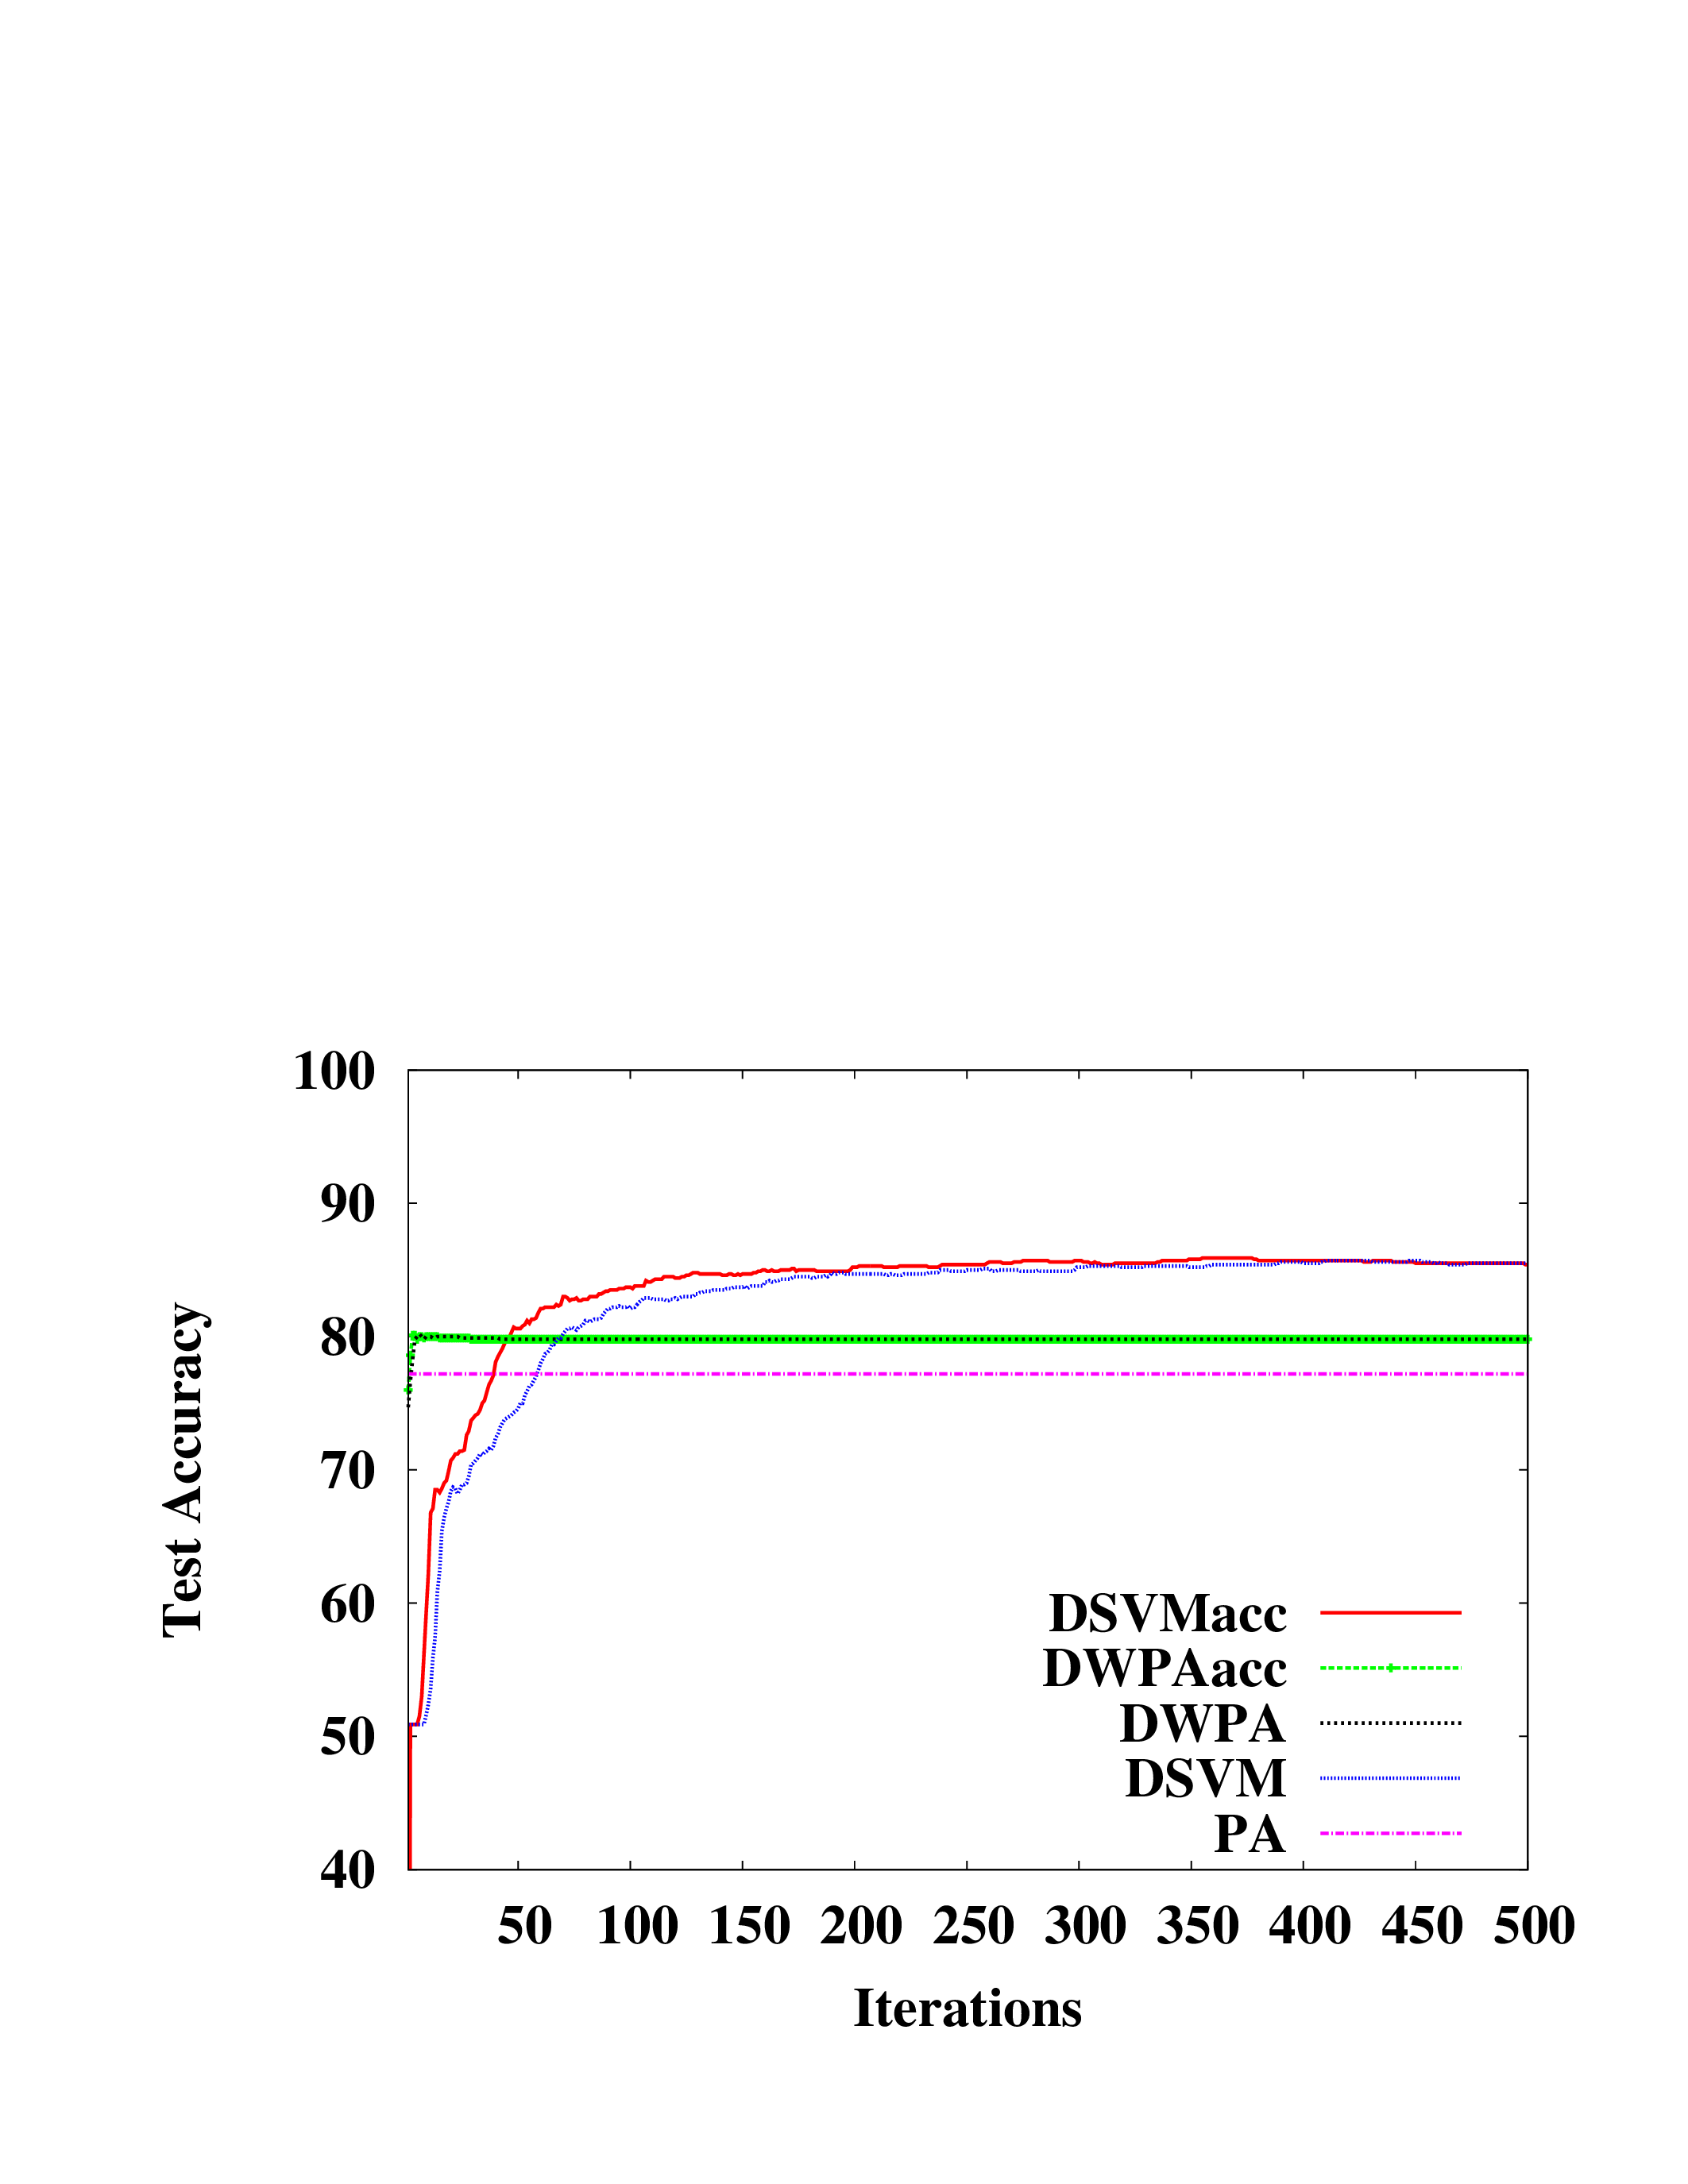}
    }
   \hspace{-.45cm}
    \subfloat[][100 partitions]{%[10 partitions]
   \includegraphics[width=0.34\linewidth]{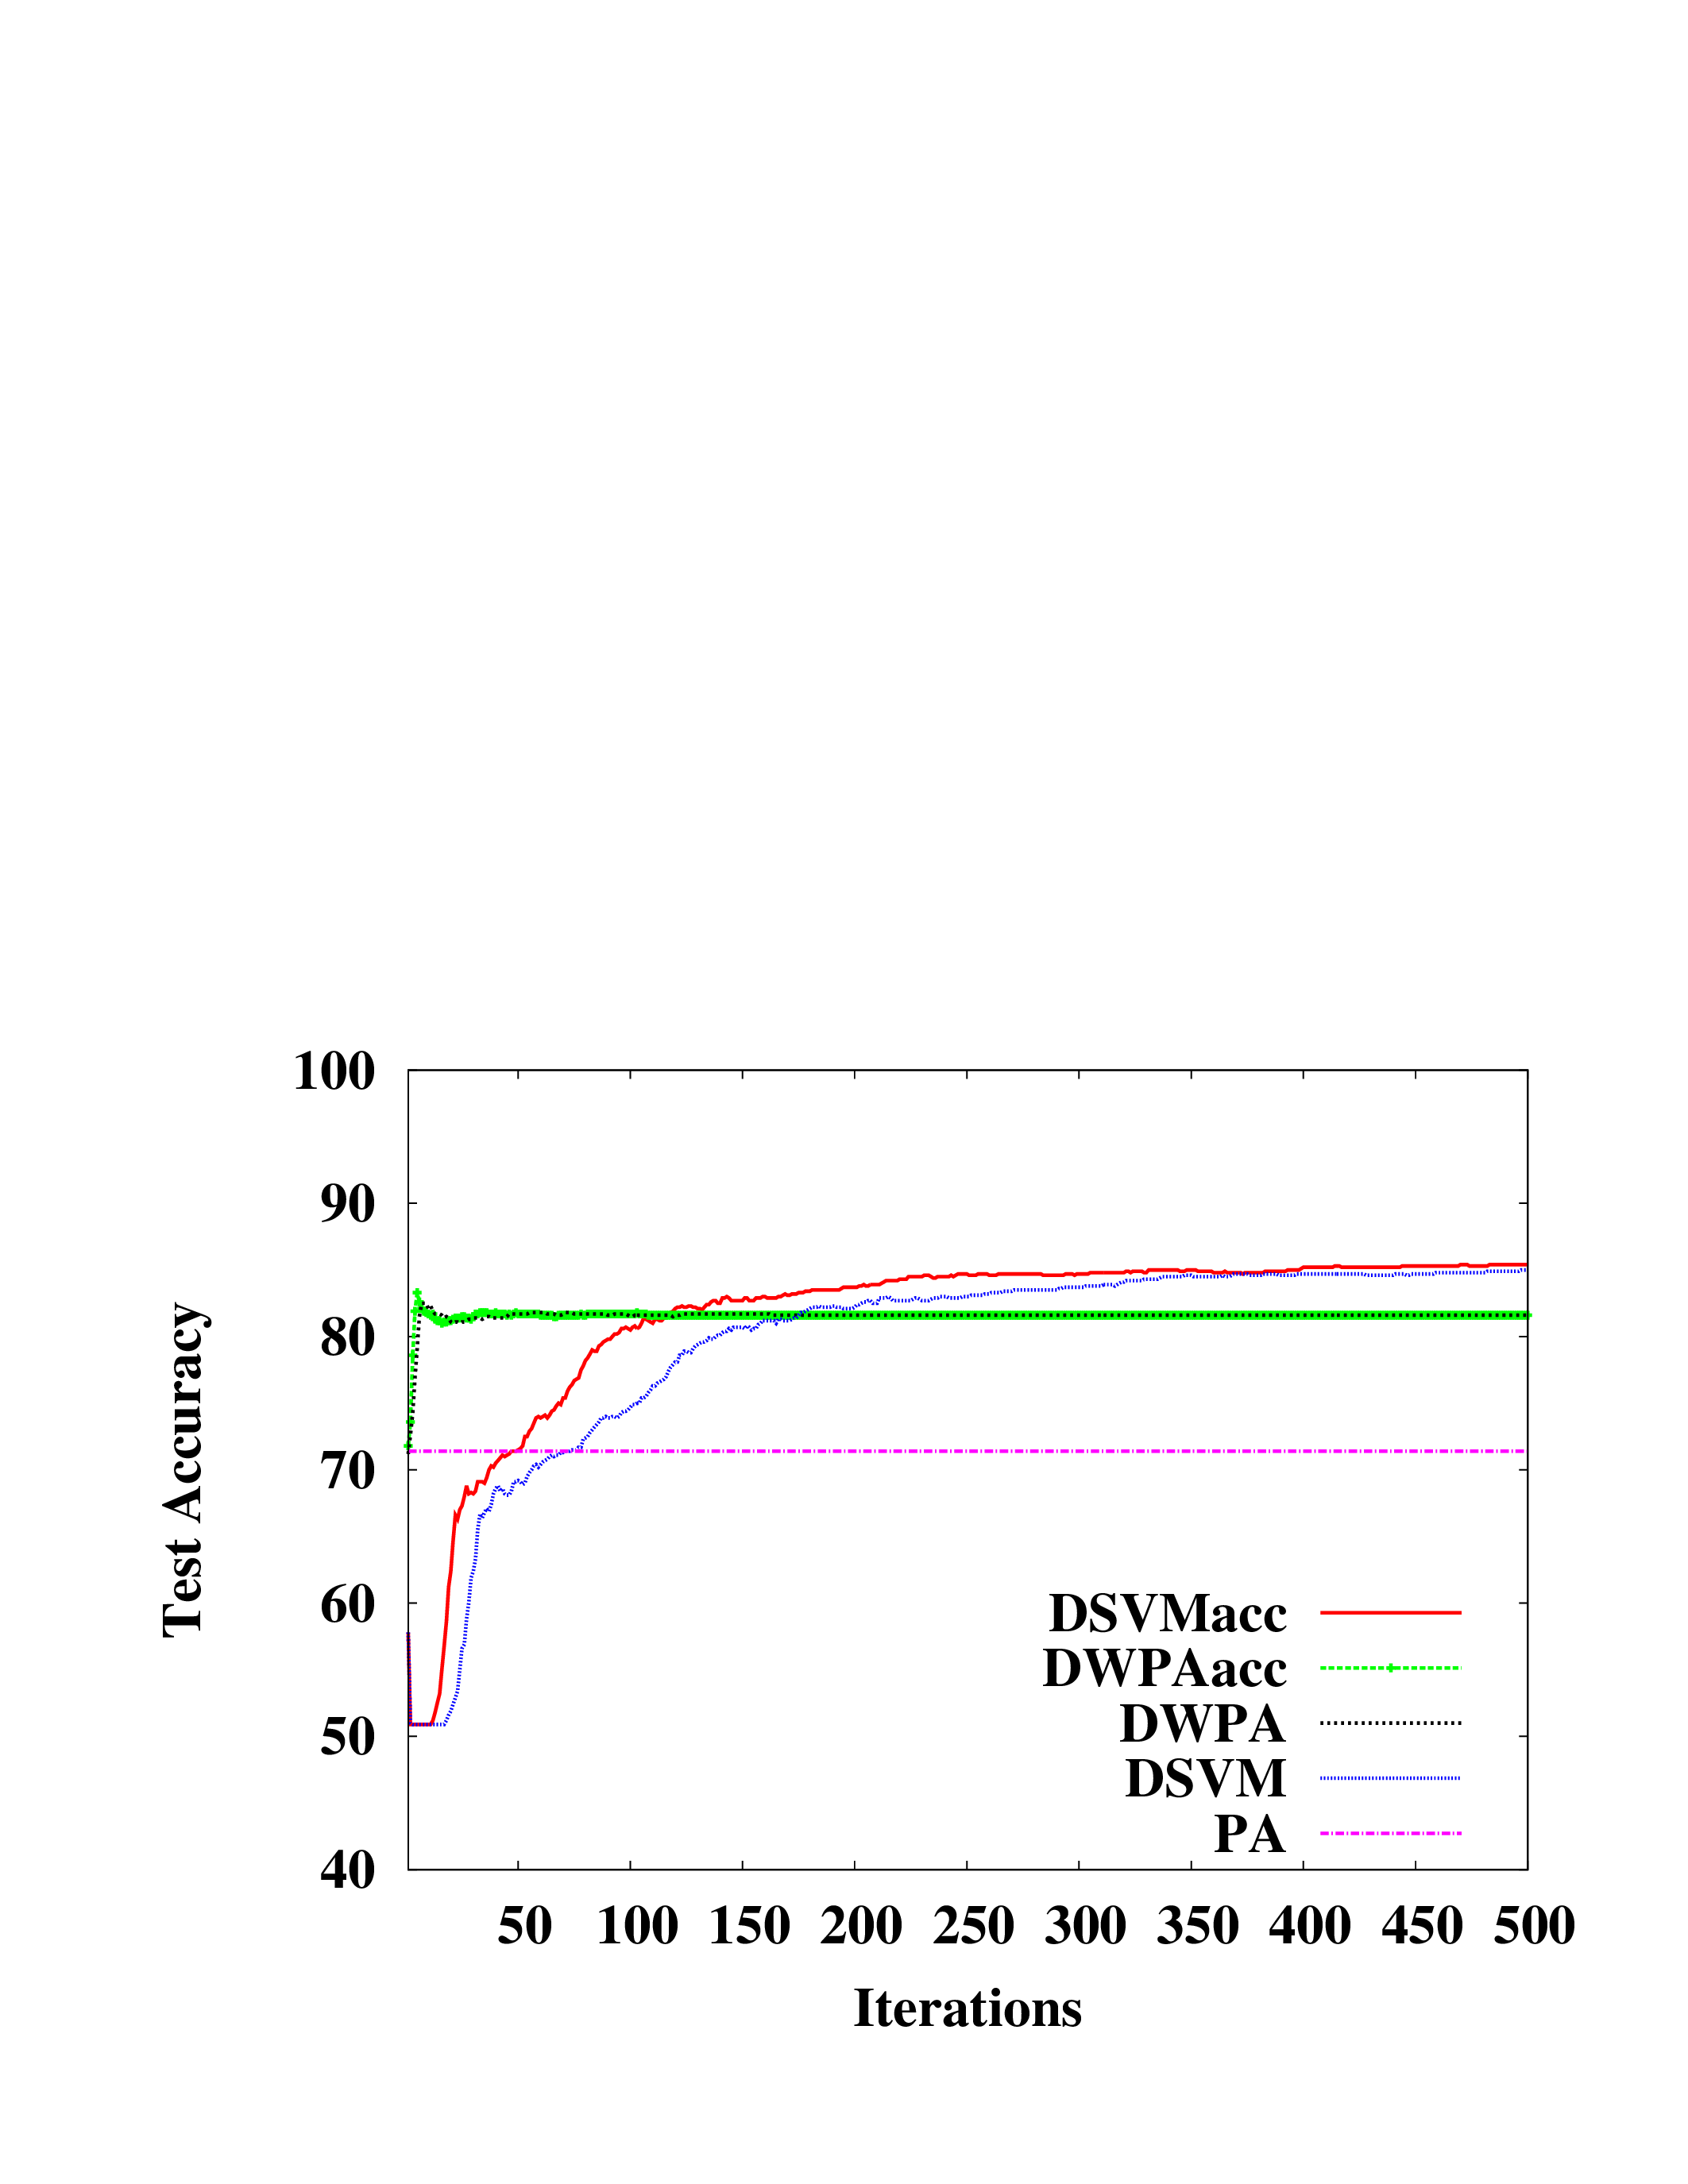}
    }
   \hspace{-.45cm}
    \subfloat[][200 partitions]{%[10 partitions]
   \includegraphics[width=0.34\linewidth]{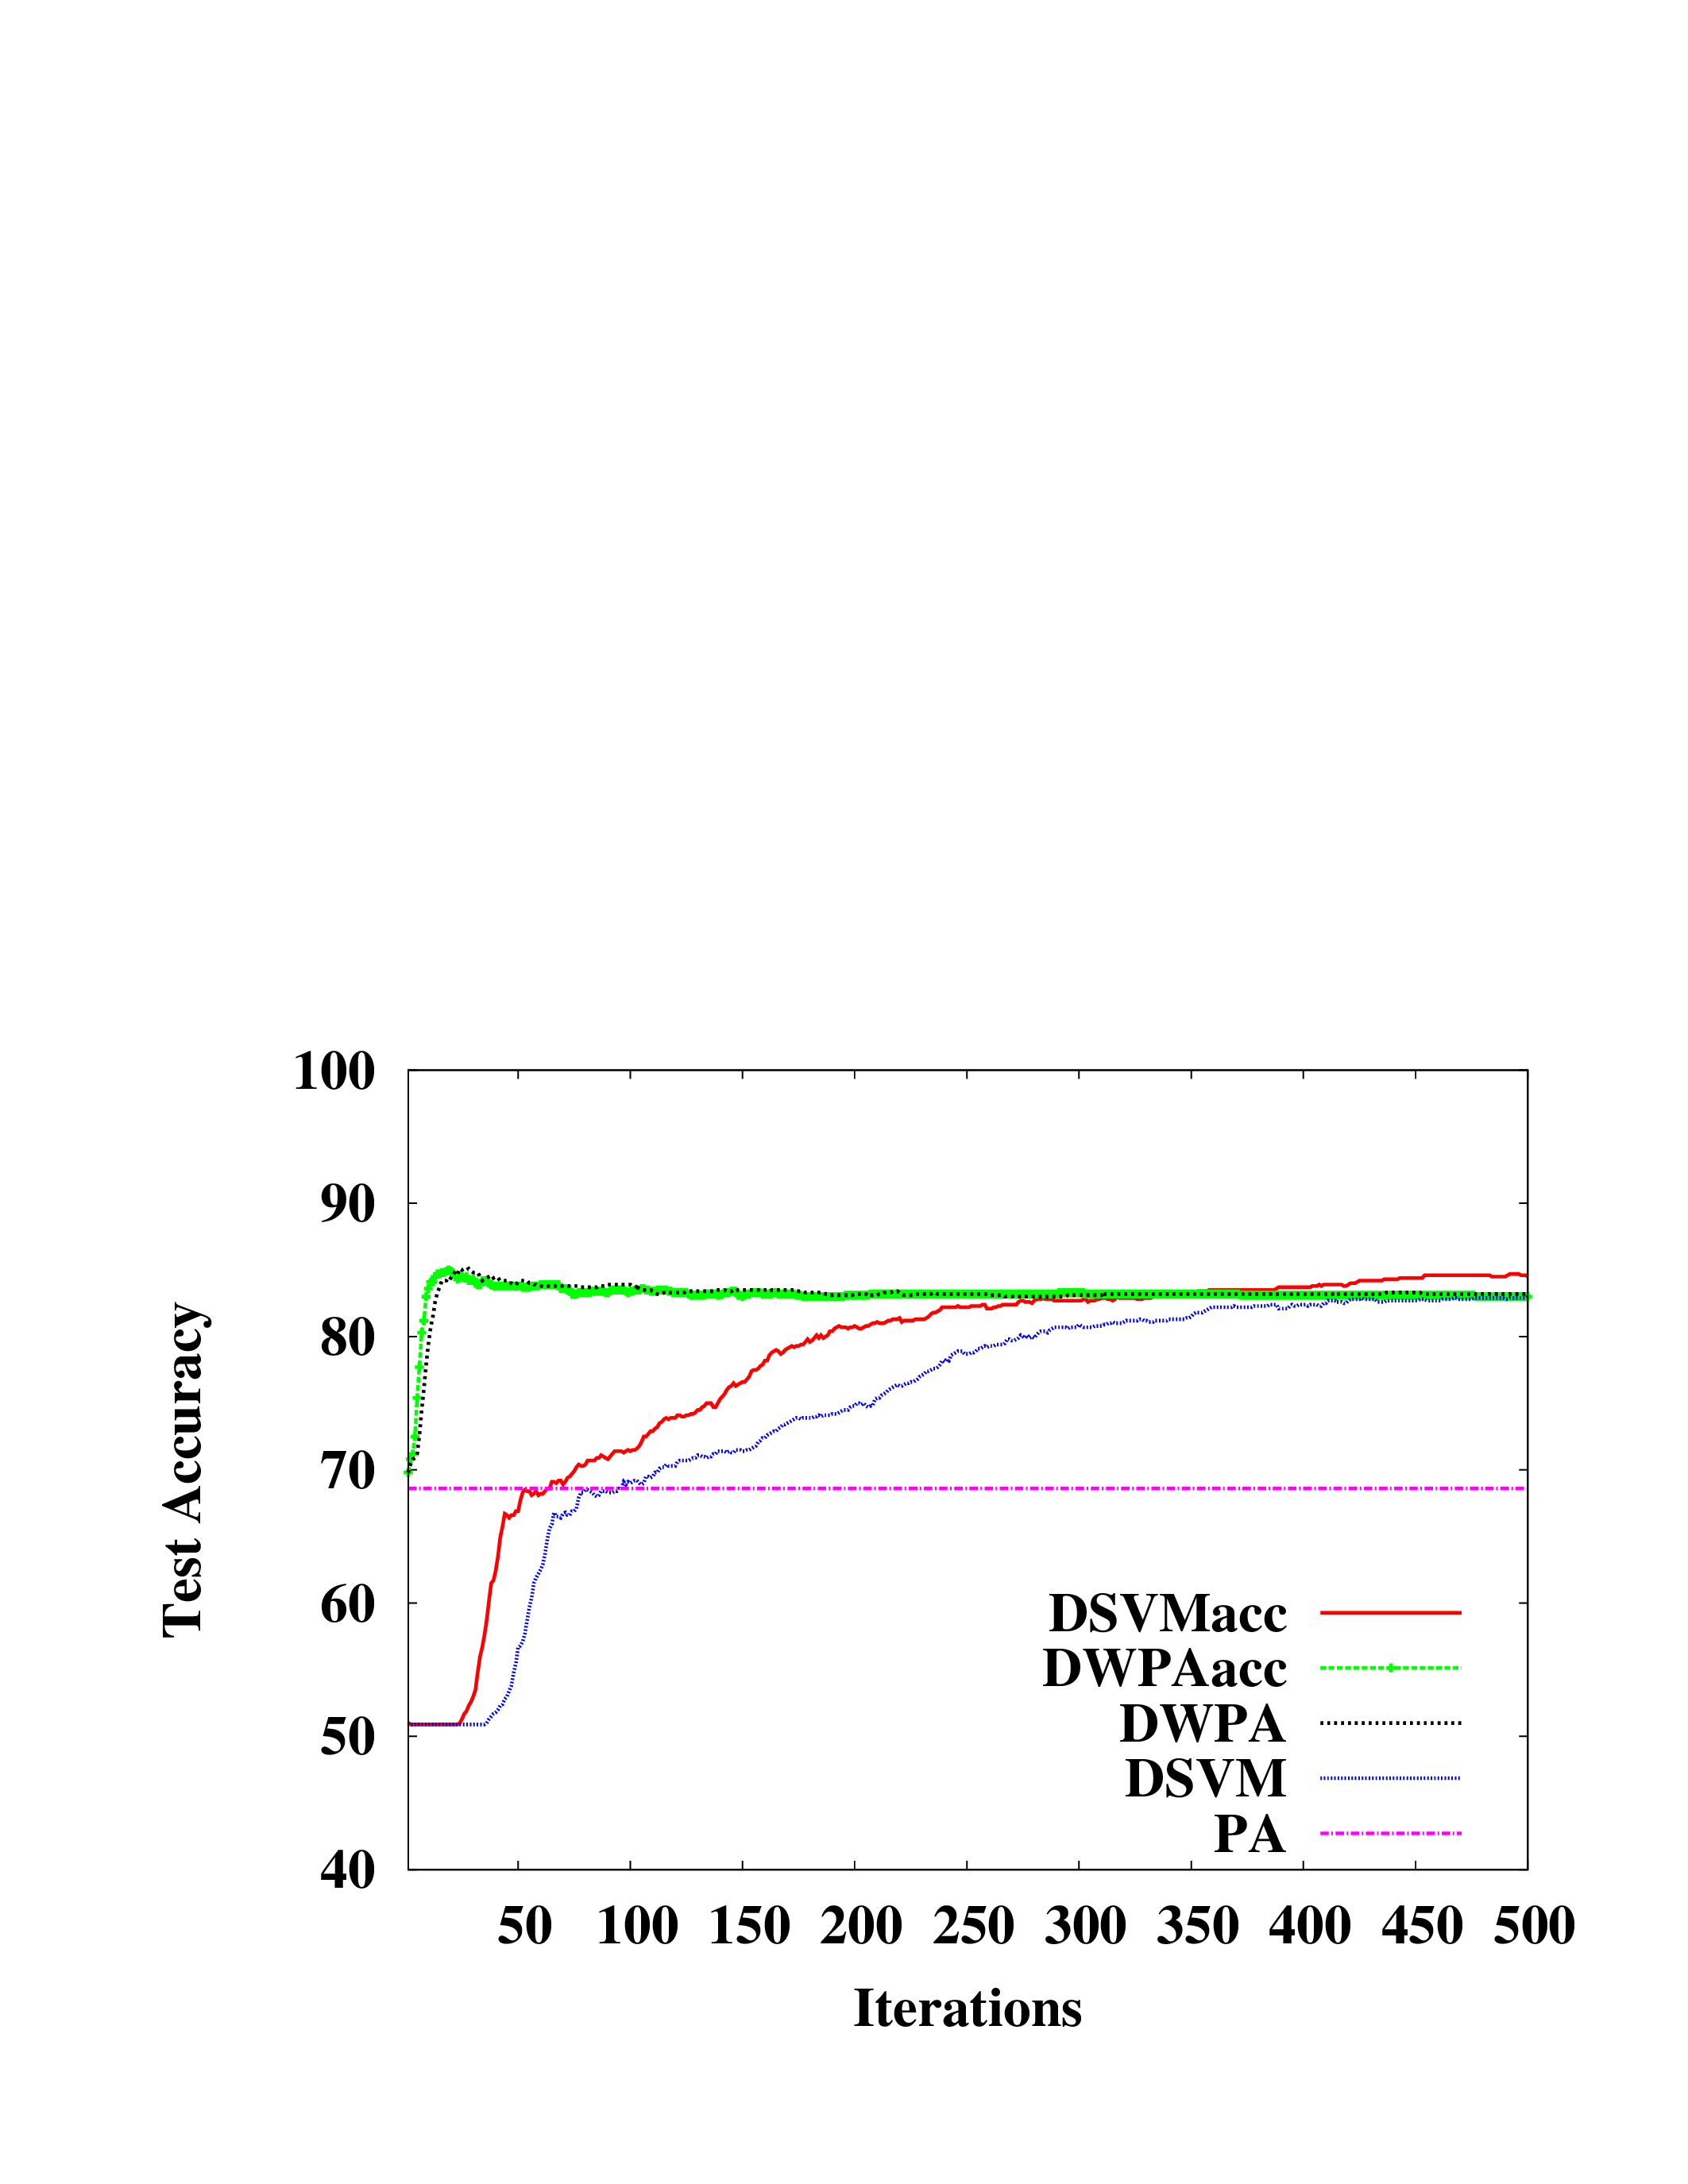}
    }
        \hspace{-.45cm}
   \subfloat[][50 partitions]{%[10 partitions]
   \includegraphics[width=0.34\linewidth]{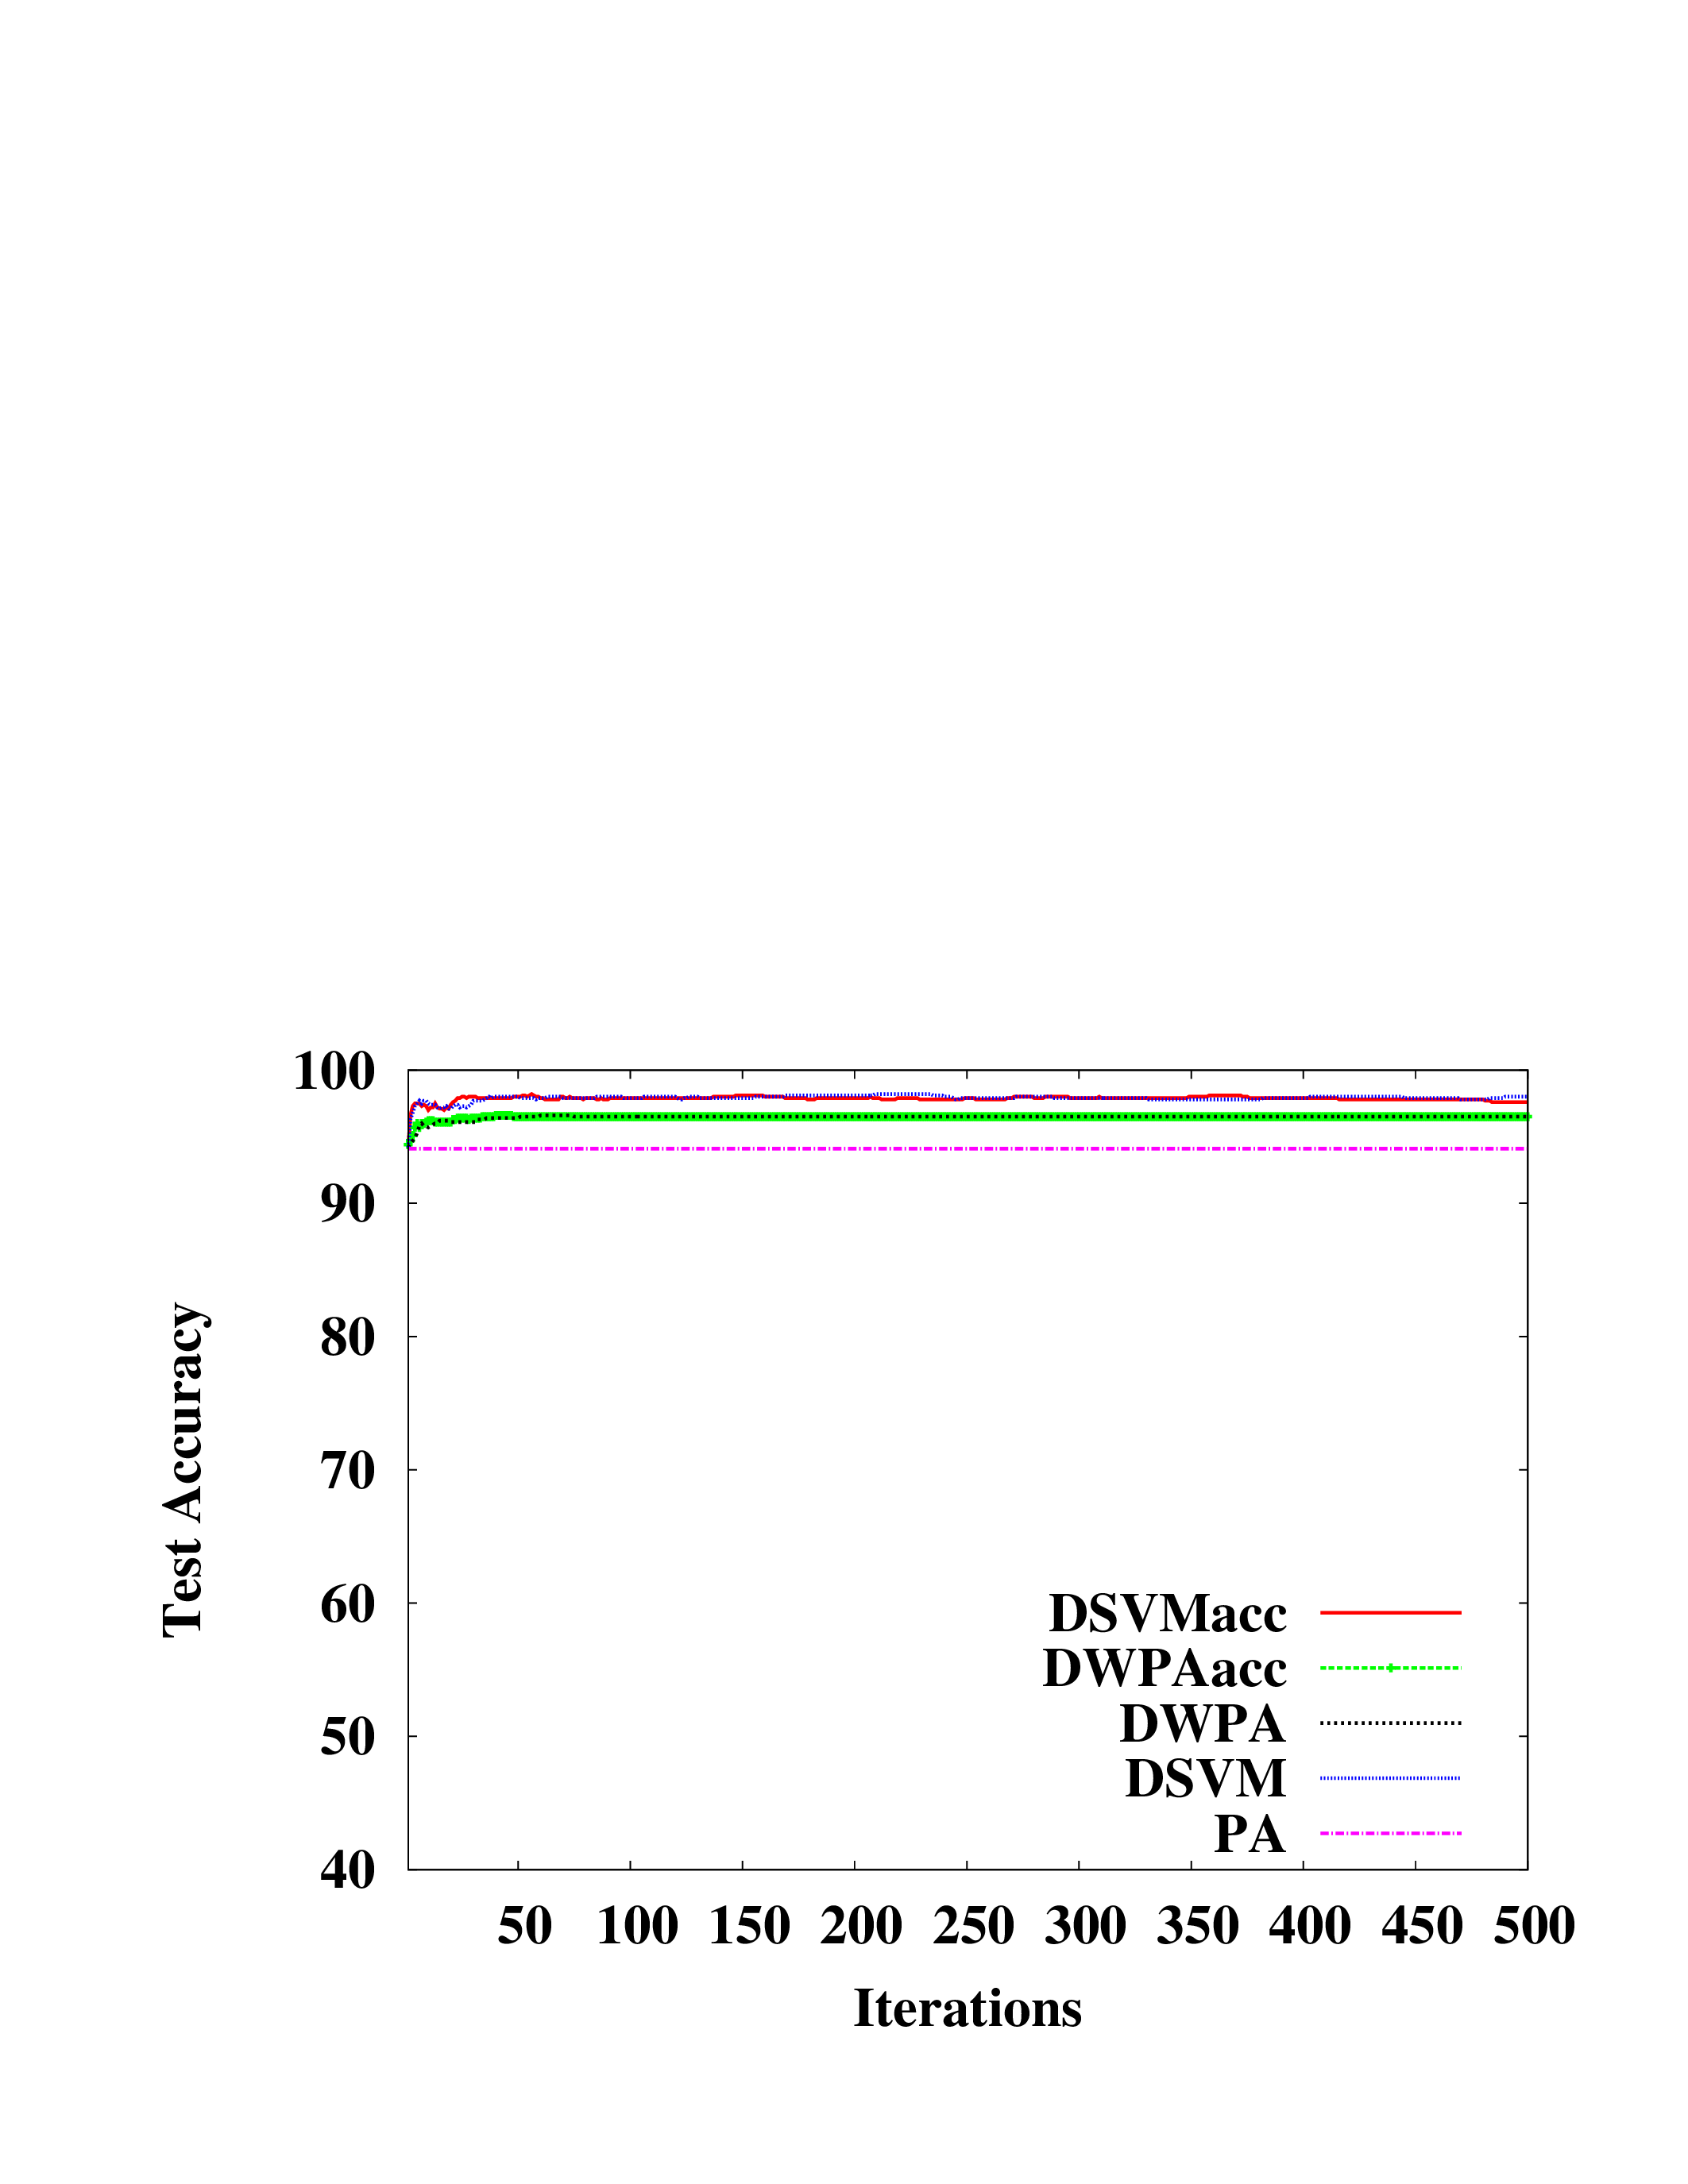}
    }
   \hspace{-.45cm}
    \subfloat[][100 partitions]{%[10 partitions]
   \includegraphics[width=0.34\linewidth]{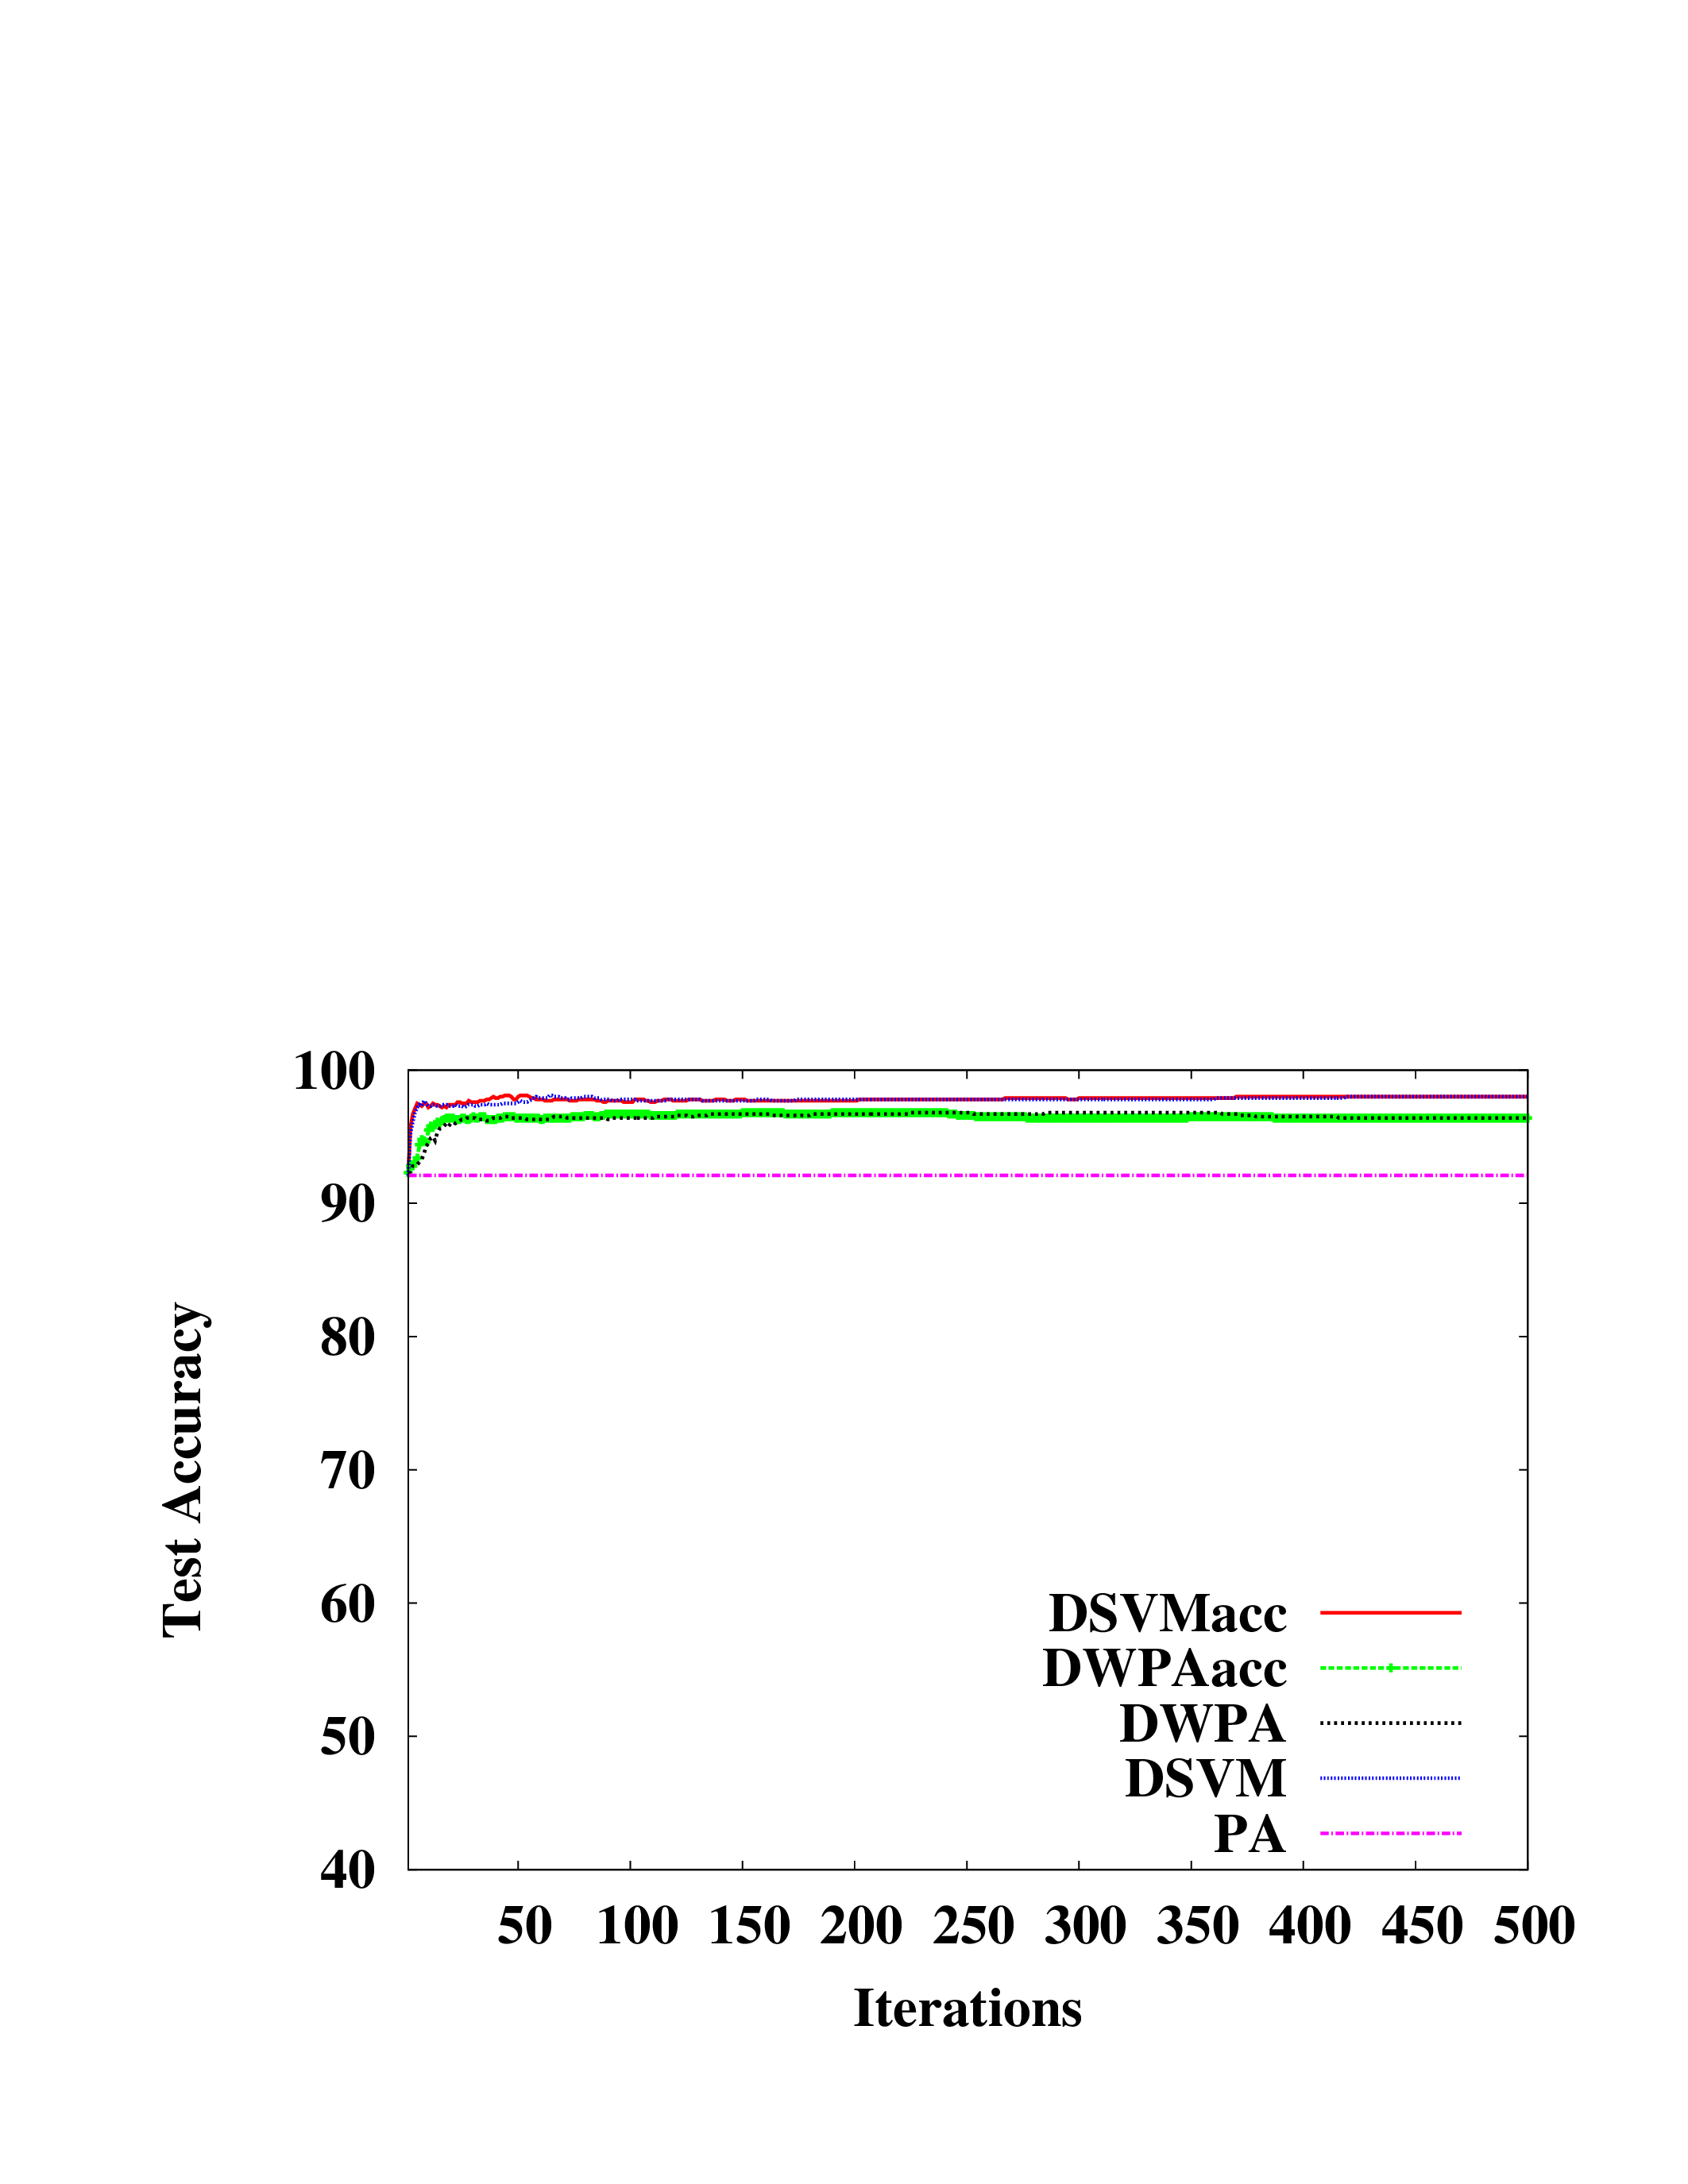}
    }
   \hspace{-.45cm}
    \subfloat[][200 partitions]{%[10 partitions]
   \includegraphics[width=0.34\linewidth]{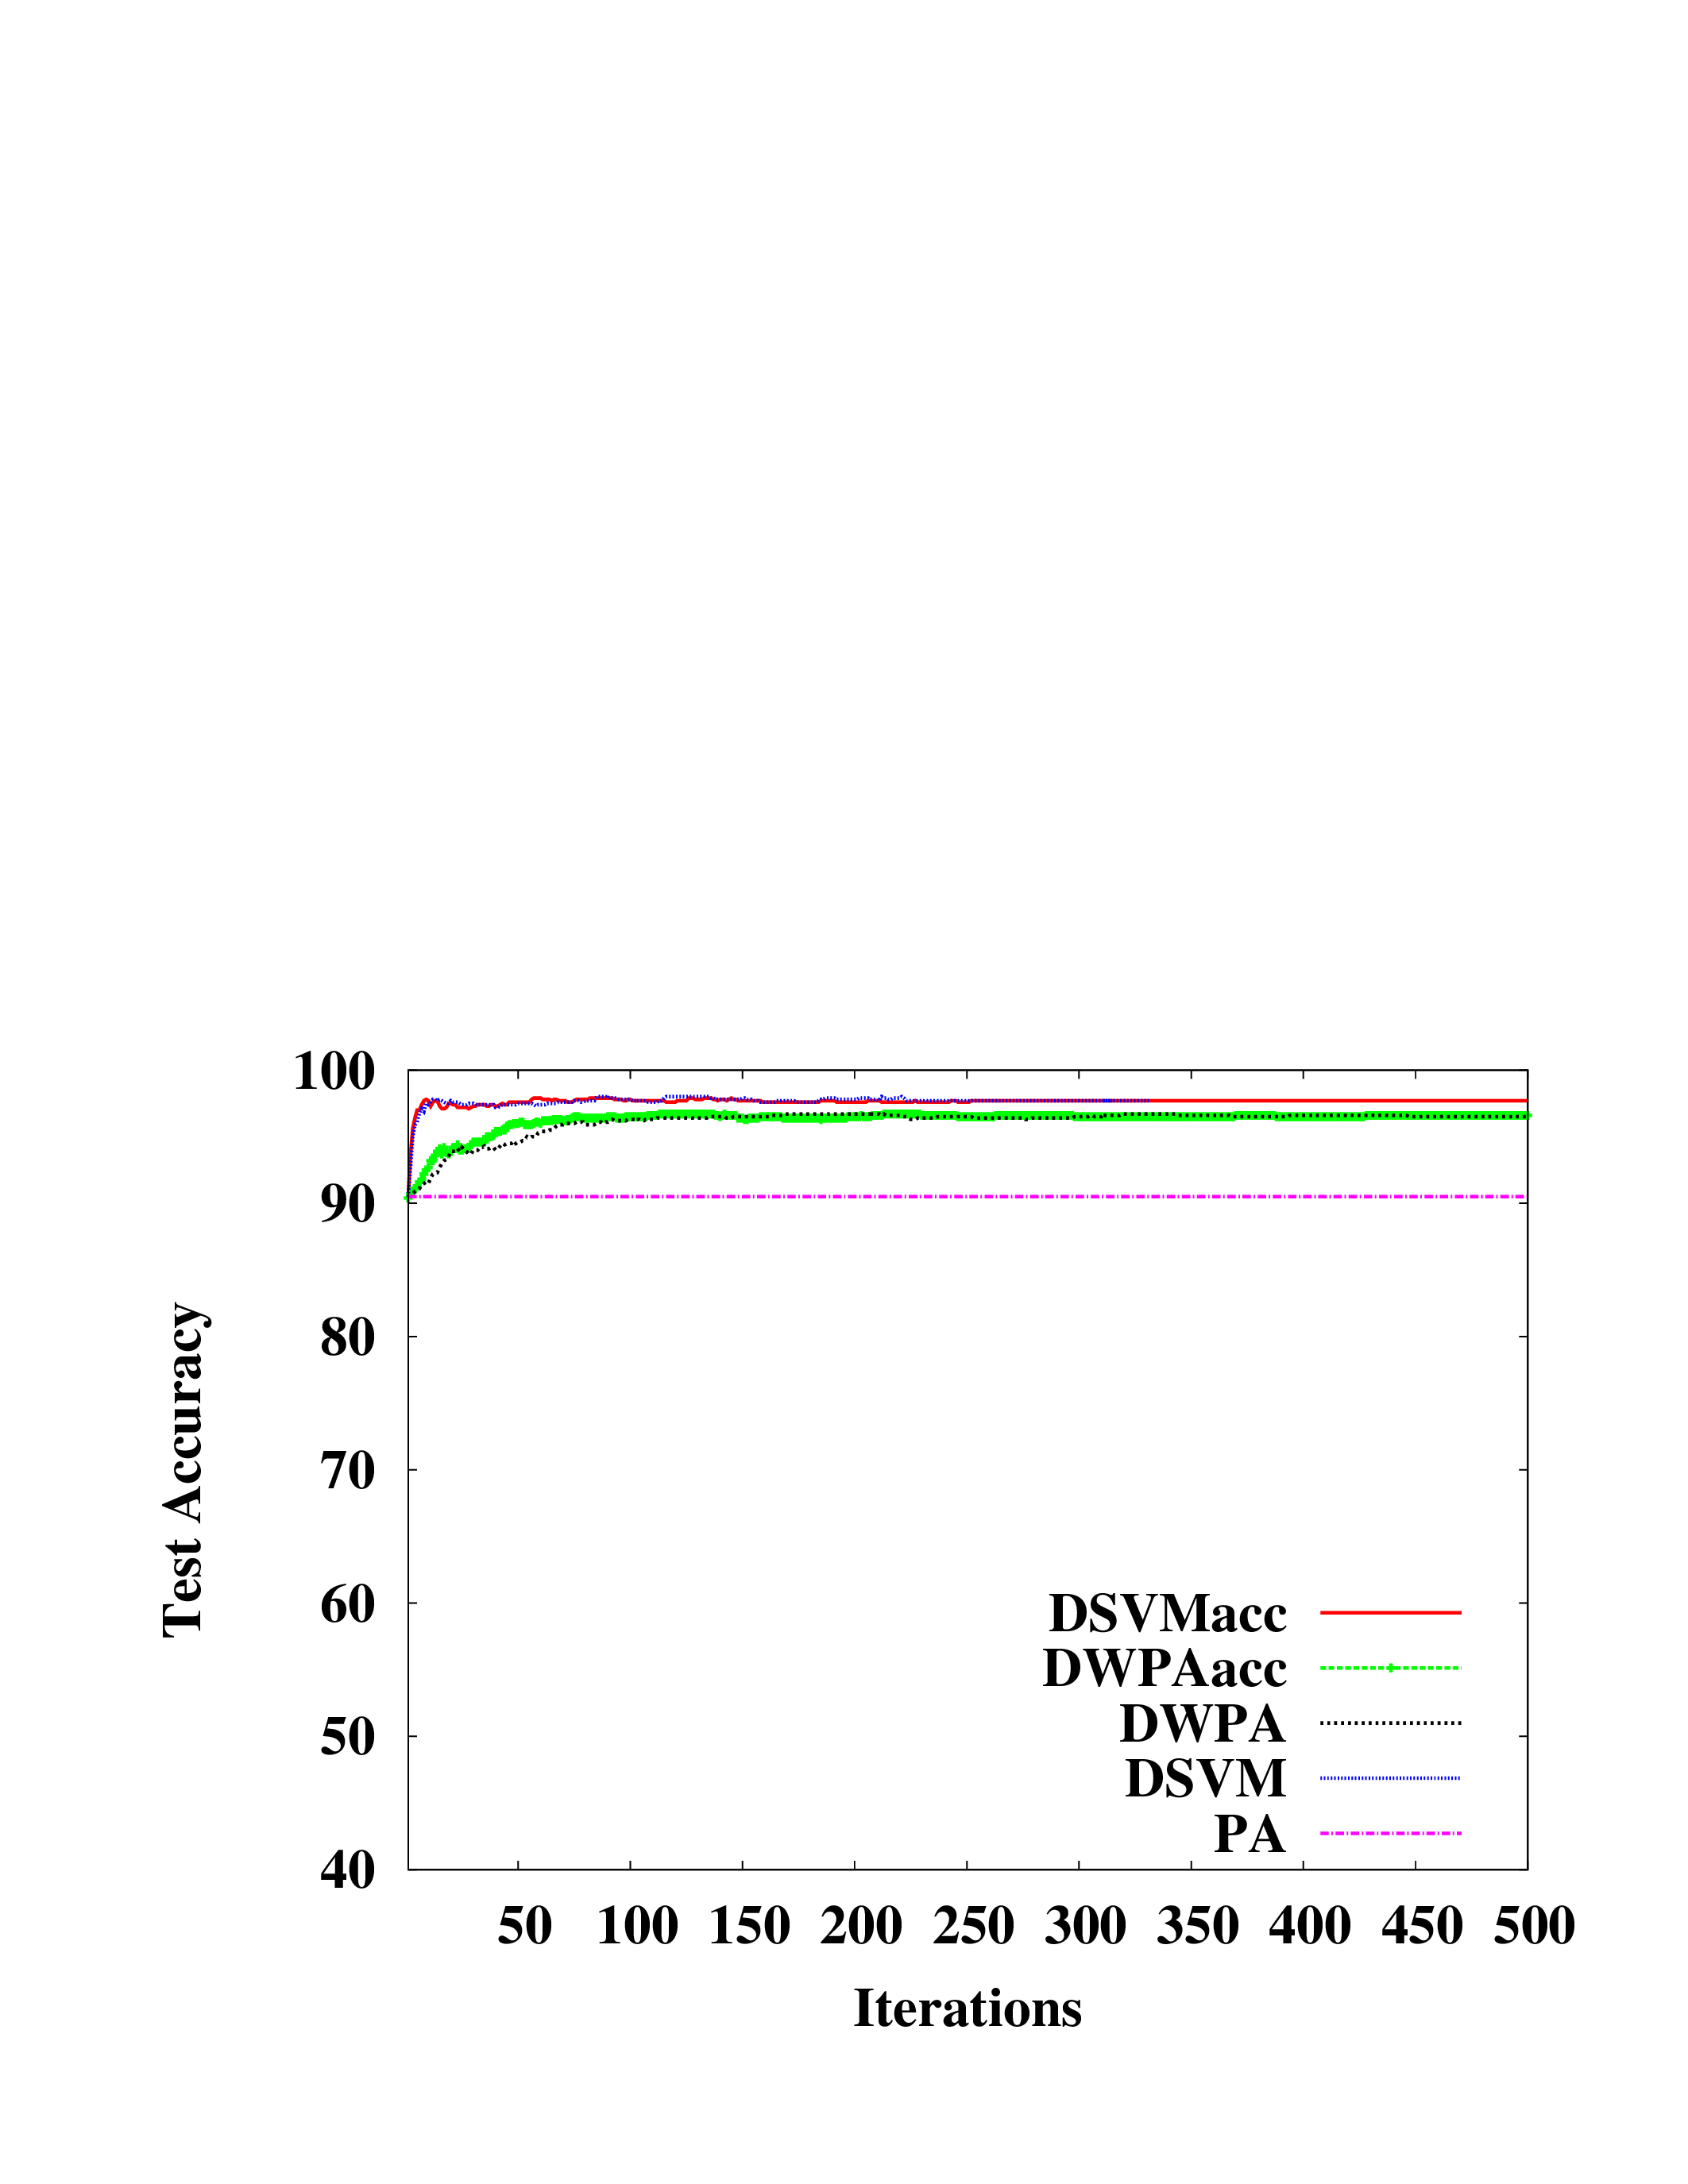}
    }
 \end{center}
 %\vspace{-0.5cm}
   \caption{\label{te}Testset accuracies for \textbf{real-sim}(top), \textbf{epsilon}(middle) and \textbf{gisette}(below)}
 \end{figure}
